# Supplementary material for: Learning Expressive Priors for Generalization and Uncertainty Estimation in Neural Networks
Source: arXiv:2307.07753 source file (2026-03-30)
Supplement: Supplementary file 1 [file results.tex]

\documentclass{standalone}
\usepackage[ansinew]{inputenc}

\usepackage{tikz_include}

\begin{document}

\begin{tikzpicture}

    \begin{groupplot}[
    group style={group size=2 by 2, y descriptions at=edge left, x descriptions at=edge bottom},
    log basis x={10},
    xlabel={Batch size},
    ylabel={Relative error},
    xmode=log
    ]
        \nextgroupplot[legend to name={CommonLegend1},legend style={legend columns=4}, ymin=-.01, ymax=1]
            \path [fill=TUMBlue, fill opacity=0.3]
            (axis cs:1,0.991297483444214)
            --(axis cs:1,0.988482475280762)
            --(axis cs:10,0.989575982093811)
            --(axis cs:100,0.989075005054474)
            --(axis cs:506,0.989341080188751)
            --(axis cs:506,0.991125285625458)
            --(axis cs:506,0.991125285625458)
            --(axis cs:100,0.99122554063797)
            --(axis cs:10,0.990574717521667)
            --(axis cs:1,0.991297483444214)
            --cycle;
            
            \path [fill=TUMAccentOrange, fill opacity=0.3]
            (axis cs:1,0.76869922876358)
            --(axis cs:1,0.575373411178589)
            --(axis cs:10,0.597745358943939)
            --(axis cs:100,0.567828416824341)
            --(axis cs:506,0.597041368484497)
            --(axis cs:506,0.70044332742691)
            --(axis cs:506,0.70044332742691)
            --(axis cs:100,0.874498724937439)
            --(axis cs:10,0.706664443016052)
            --(axis cs:1,0.76869922876358)
            --cycle;
            
            \path [fill=TUMAccentGreen, fill opacity=0.3]
            (axis cs:1,0.570764482021332)
            --(axis cs:1,0.482513457536697)
            --(axis cs:10,0.465409487485886)
            --(axis cs:100,0.451181083917618)
            --(axis cs:506,0.430667906999588)
            --(axis cs:506,0.486570090055466)
            --(axis cs:506,0.486570090055466)
            --(axis cs:100,0.502846002578735)
            --(axis cs:10,0.513382375240326)
            --(axis cs:1,0.570764482021332)
            --cycle;
            
            \path [fill=TUMDarkGray, fill opacity=0.3]
            (axis cs:1,0.504947543144226)
            --(axis cs:1,0.446379810571671)
            --(axis cs:10,0.460807621479034)
            --(axis cs:100,0.425737589597702)
            --(axis cs:506,0.430667906999588)
            --(axis cs:506,0.486570090055466)
            --(axis cs:506,0.486570090055466)
            --(axis cs:100,0.477021485567093)
            --(axis cs:10,0.503044486045837)
            --(axis cs:1,0.504947543144226)
            --cycle;
            
            \addplot [very thick, TUMBlue, dotted]
            table {%
            1 0.990160930156708
            10 0.990065634250641
            100 0.990156894922256
            506 0.990091449022293
            };
            \addlegendentry{Diagonal}
            \addplot [very thick, TUMAccentOrange, loosely dashed]
            table {%
            1 0.644238209724426
            10 0.642899233102799
            100 0.674370324611664
            506 0.647445183992386
            };
            \addlegendentry{K-FAC}
            \addplot [very thick, TUMAccentGreen, dashdotted]
            table {%
            1 0.534151205420494
            10 0.49739017188549
            100 0.482025536894798
            506 0.464413401484489
            };
            \addlegendentry{K-FOC\_approx}
            \addplot [very thick, TUMDarkGray]
            table {%
            1 0.469396069645882
            10 0.482338461279869
            100 0.460488444566727
            506 0.464413401484489
            };
            \addlegendentry{K-FOC\_running}

        \nextgroupplot[ymin=-.01, ymax=1]
            \path [fill=TUMBlue, fill opacity=0.3]
            (axis cs:1,0.967395782470703)
            --(axis cs:1,0.963500797748566)
            --(axis cs:10,0.96381664276123)
            --(axis cs:100,0.964037120342255)
            --(axis cs:506,0.963381886482239)
            --(axis cs:506,0.967442393302917)
            --(axis cs:506,0.967442393302917)
            --(axis cs:100,0.967752695083618)
            --(axis cs:10,0.967956125736237)
            --(axis cs:1,0.967395782470703)
            --cycle;
            
            \path [fill=TUMAccentOrange, fill opacity=0.3]
            (axis cs:1,0.143594533205032)
            --(axis cs:1,0.0599139668047428)
            --(axis cs:10,0.0477773435413837)
            --(axis cs:100,0.0809624195098877)
            --(axis cs:506,0.0634049028158188)
            --(axis cs:506,0.167380213737488)
            --(axis cs:506,0.167380213737488)
            --(axis cs:100,0.231848135590553)
            --(axis cs:10,0.173649862408638)
            --(axis cs:1,0.143594533205032)
            --cycle;
            
            \path [fill=TUMAccentGreen, fill opacity=0.3]
            (axis cs:1,0.326390415430069)
            --(axis cs:1,0.221594408154488)
            --(axis cs:10,0.0786982849240303)
            --(axis cs:100,0.0539965629577637)
            --(axis cs:506,7.89041735060891e-07)
            --(axis cs:506,2.10441885428736e-05)
            --(axis cs:506,2.10441885428736e-05)
            --(axis cs:100,0.157867476344109)
            --(axis cs:10,0.179624795913696)
            --(axis cs:1,0.326390415430069)
            --cycle;
            
            \path [fill=TUMDarkGray, fill opacity=0.3]
            (axis cs:1,0.00781585089862347)
            --(axis cs:1,0.00271570100449026)
            --(axis cs:10,0.000910790229681879)
            --(axis cs:100,0.000323680025758222)
            --(axis cs:506,7.89041735060891e-07)
            --(axis cs:506,2.10441885428736e-05)
            --(axis cs:506,2.10441885428736e-05)
            --(axis cs:100,0.000694891554303467)
            --(axis cs:10,0.00279312790371478)
            --(axis cs:1,0.00781585089862347)
            --cycle;
            
            \addplot [very thick, TUMBlue, dotted]
            table {%
            1 0.965438222885132
            10 0.965842771530151
            100 0.966155046224594
            506 0.965603810548782
            };
            \addplot [very thick, TUMAccentOrange, loosely dashed]
            table {%
            1 0.100710521265864
            10 0.103799131885171
            100 0.122188185155392
            506 0.0954830206930637
            };
            \addplot [very thick, TUMAccentGreen, dashdotted]
            table {%
            1 0.286819465458393
            10 0.110696902871132
            100 0.0918451357632875
            506 8.37024370525796e-06
            };
            \addplot [very thick, TUMDarkGray]
            table {%
            1 0.00492819922510535
            10 0.00140488335164264
            100 0.000452783974469639
            506 8.37024370525796e-06
            };

        \nextgroupplot
            \path [fill=TUMAccentGreen, fill opacity=0.3]
            (axis cs:1,0.927799999713898)
            --(axis cs:1,0.580099999904633)
            --(axis cs:10,0.549399971961975)
            --(axis cs:100,0.512899994850159)
            --(axis cs:1000,0.508800029754639)
            --(axis cs:1000,0.683600008487701)
            --(axis cs:1000,0.683600008487701)
            --(axis cs:100,0.937200009822845)
            --(axis cs:10,0.969500005245209)
            --(axis cs:1,0.927799999713898)
            --cycle;
            
            \path [fill=TUMBlue, fill opacity=0.3]
            (axis cs:1,0.982147872447968)
            --(axis cs:1,0.980560839176178)
            --(axis cs:10,0.980370998382568)
            --(axis cs:100,0.981037437915802)
            --(axis cs:1000,0.981064200401306)
            --(axis cs:1000,0.981797933578491)
            --(axis cs:1000,0.981797933578491)
            --(axis cs:100,0.982132315635681)
            --(axis cs:10,0.981944739818573)
            --(axis cs:1,0.982147872447968)
            --cycle;
            
            \path [fill=TUMAccentOrange, fill opacity=0.3]
            (axis cs:1,0.965794146060944)
            --(axis cs:1,0.963271737098694)
            --(axis cs:10,0.963302373886108)
            --(axis cs:100,0.962383329868317)
            --(axis cs:1000,0.96306437253952)
            --(axis cs:1000,0.96613073348999)
            --(axis cs:1000,0.96613073348999)
            --(axis cs:100,0.966456353664398)
            --(axis cs:10,0.966358006000519)
            --(axis cs:1,0.965794146060944)
            --cycle;
            
            \path [fill=TUMDarkGray, fill opacity=0.3]
            (axis cs:1,0.55618143081665)
            --(axis cs:1,0.506643652915955)
            --(axis cs:10,0.507703185081482)
            --(axis cs:100,0.509818375110626)
            --(axis cs:1000,0.508744835853577)
            --(axis cs:1000,0.528092563152313)
            --(axis cs:1000,0.528092563152313)
            --(axis cs:100,0.518947839736938)
            --(axis cs:10,0.541475772857666)
            --(axis cs:1,0.55618143081665)
            --cycle;
            
            \addplot [very thick, TUMBlue, dotted]
            table {%
            1 0.981607913970947
            10 0.981380820274353
            100 0.981556594371796
            1000 0.981422901153564
            };
            \addplot [very thick, TUMAccentOrange, loosely dashed]
            table {%
            1 0.964541137218475
            10 0.964732944965363
            100 0.964760780334473
            1000 0.964657783508301
            };
            \addplot [very thick, TUMAccentGreen, dashdotted]
            table {%
            1 0.64504998922348
            10 0.721610009670258
            100 0.608579993247986
            1000 0.533749997615814
            };
            \addplot [very thick, TUMDarkGray]
            table {%
            1 0.524177074432373
            10 0.521301507949829
            100 0.513801395893097
            1000 0.516801178455353
            };

        \nextgroupplot
            \path [fill=TUMAccentGreen, fill opacity=0.3]
            (axis cs:1,1.0003000497818)
            --(axis cs:1,0.661499977111816)
            --(axis cs:10,0.649600028991699)
            --(axis cs:100,0.633899986743927)
            --(axis cs:1000,0.621800005435944)
            --(axis cs:1000,0.99099999666214)
            --(axis cs:1000,0.99099999666214)
            --(axis cs:100,0.996200025081635)
            --(axis cs:10,0.99260002374649)
            --(axis cs:1,1.0003000497818)
            --cycle;
            
            \path [fill=TUMBlue, fill opacity=0.3]
            (axis cs:1,0.992236614227295)
            --(axis cs:1,0.991462409496307)
            --(axis cs:10,0.991383612155914)
            --(axis cs:100,0.991532742977142)
            --(axis cs:1000,0.991503119468689)
            --(axis cs:1000,0.991781115531921)
            --(axis cs:1000,0.991781115531921)
            --(axis cs:100,0.991807758808136)
            --(axis cs:10,0.99201226234436)
            --(axis cs:1,0.992236614227295)
            --cycle;
            
            \path [fill=TUMAccentOrange, fill opacity=0.3]
            (axis cs:1,0.847472310066223)
            --(axis cs:1,0.831174969673157)
            --(axis cs:10,0.828693211078644)
            --(axis cs:100,0.828133463859558)
            --(axis cs:1000,0.826321244239807)
            --(axis cs:1000,0.836274147033691)
            --(axis cs:1000,0.836274147033691)
            --(axis cs:100,0.836199522018433)
            --(axis cs:10,0.836920499801636)
            --(axis cs:1,0.847472310066223)
            --cycle;
            
            \path [fill=TUMDarkGray, fill opacity=0.3]
            (axis cs:1,0.661402463912964)
            --(axis cs:1,0.643310606479645)
            --(axis cs:10,0.634492993354797)
            --(axis cs:100,0.626134395599365)
            --(axis cs:1000,0.621075689792633)
            --(axis cs:1000,0.631477415561676)
            --(axis cs:1000,0.631477415561676)
            --(axis cs:100,0.639983177185059)
            --(axis cs:10,0.64990770816803)
            --(axis cs:1,0.661402463912964)
            --cycle;
            
            \addplot [very thick, TUMAccentGreen, dashdotted]
            table {%
            1 0.81752997636795
            10 0.821550011634827
            100 0.752699971199036
            1000 0.663929998874664
            };
            \addplot [very thick, TUMBlue, dotted]
            table {%
            1 0.991794407367706
            10 0.991709589958191
            100 0.991657614707947
            1000 0.991664290428162
            };
            \addplot [very thick, TUMAccentOrange, loosely dashed]
            table {%
            1 0.837280094623566
            10 0.832380890846252
            100 0.831797242164612
            1000 0.832187294960022
            };
            \addplot [very thick, TUMDarkGray]
            table {%
            1 0.651285827159882
            10 0.642952144145966
            100 0.634984910488129
            1000 0.627077698707581
            };  
    \end{groupplot}

    \path (group c1r2.south east) -- node[below=1.2cm]{\pgfplotslegendfromname{CommonLegend1}} (group c2r2.south west);
\end{tikzpicture}

\end{document}
