# Supplementary material for: Learning Expressive Priors for Generalization and Uncertainty Estimation in Neural Networks
Source: arXiv:2307.07753 source file (2026-03-30)
Supplement: Supplementary file 2 [file results_further.tex]

\documentclass{standalone}
\usepackage[ansinew]{inputenc}

\usepackage{tikz_include}

\begin{document}

\begin{tikzpicture}
    
    \begin{groupplot}[
    group style={group size=2 by 2, y descriptions at=edge left, x descriptions at=edge bottom},
    log basis x={10},
    xlabel={Batch size},
    ylabel={Relative error},
    xmode=log
    ]
        \nextgroupplot[legend to name={CommonLegend2},legend style={legend columns=4}, ymin=-.01, ymax=1]
            \path [fill=TUMBlue, fill opacity=0.3]
            (axis cs:1,0.989152371883392)
            --(axis cs:1,0.988199830055237)
            --(axis cs:10,0.988359272480011)
            --(axis cs:100,0.988220870494843)
            --(axis cs:1030,0.988284528255463)
            --(axis cs:1030,0.989518105983734)
            --(axis cs:1030,0.989518105983734)
            --(axis cs:100,0.988947212696075)
            --(axis cs:10,0.989346444606781)
            --(axis cs:1,0.989152371883392)
            --cycle;
            
            \path [fill=TUMAccentOrange, fill opacity=0.3]
            (axis cs:1,0.408934593200684)
            --(axis cs:1,0.374109923839569)
            --(axis cs:10,0.365101218223572)
            --(axis cs:100,0.368731707334518)
            --(axis cs:1030,0.365104049444199)
            --(axis cs:1030,0.438257157802582)
            --(axis cs:1030,0.438257157802582)
            --(axis cs:100,0.443823844194412)
            --(axis cs:10,0.409665435552597)
            --(axis cs:1,0.408934593200684)
            --cycle;
            
            \path [fill=TUMAccentGreen, fill opacity=0.3]
            (axis cs:1,0.530634343624115)
            --(axis cs:1,0.443665087223053)
            --(axis cs:10,0.359032958745956)
            --(axis cs:100,0.332548141479492)
            --(axis cs:1030,0.304121226072311)
            --(axis cs:1030,0.358720451593399)
            --(axis cs:1030,0.358720451593399)
            --(axis cs:100,0.35747754573822)
            --(axis cs:10,0.410523742437363)
            --(axis cs:1,0.530634343624115)
            --cycle;
            
            \path [fill=TUMDarkGray, fill opacity=0.3]
            (axis cs:1,0.354820221662521)
            --(axis cs:1,0.319812178611755)
            --(axis cs:10,0.323164731264114)
            --(axis cs:100,0.32932785153389)
            --(axis cs:1030,0.304121285676956)
            --(axis cs:1030,0.358720451593399)
            --(axis cs:1030,0.358720451593399)
            --(axis cs:100,0.349448829889297)
            --(axis cs:10,0.357538282871246)
            --(axis cs:1,0.354820221662521)
            --cycle;
            
            \addplot [very thick, TUMBlue, dotted]
            table {%
            1 0.988733613491058
            10 0.988684004545212
            100 0.988731622695923
            1030 0.988813656568527
            };
            \addlegendentry{Diagonal}
            \addplot [very thick, TUMAccentOrange, loosely dashed]
            table {%
            1 0.387938216328621
            10 0.379789158701897
            100 0.387797725200653
            1030 0.389929684996605
            };
            \addlegendentry{K-FAC}
            \addplot [very thick, TUMAccentGreen, dashdotted]
            table {%
            1 0.485574772953987
            10 0.378320488333702
            100 0.344923263788223
            1030 0.333011090755463
            };
            \addlegendentry{K-FOC\_approx}
            \addplot [very thick, TUMDarkGray]
            table {%
            1 0.34141381084919
            10 0.34062032699585
            100 0.339495086669922
            1030 0.333011093735695
            };
            \addlegendentry{K-FOC\_running}

        \nextgroupplot[ymin=-.01, ymax=1]
            \path [fill=TUMBlue, fill opacity=0.3]
            (axis cs:1,0.971454322338104)
            --(axis cs:1,0.97032755613327)
            --(axis cs:10,0.970102369785309)
            --(axis cs:100,0.970595300197601)
            --(axis cs:1030,0.970169425010681)
            --(axis cs:1030,0.972084701061249)
            --(axis cs:1030,0.972084701061249)
            --(axis cs:100,0.971342742443085)
            --(axis cs:10,0.971745073795319)
            --(axis cs:1,0.971454322338104)
            --cycle;
            
            \path [fill=TUMAccentOrange, fill opacity=0.3]
            (axis cs:1,0.110392443835735)
            --(axis cs:1,0.0468147248029709)
            --(axis cs:10,0.0509092397987843)
            --(axis cs:100,0.0457135997712612)
            --(axis cs:1030,0.0512361116707325)
            --(axis cs:1030,0.122465007007122)
            --(axis cs:1030,0.122465007007122)
            --(axis cs:100,0.142586410045624)
            --(axis cs:10,0.182065859436989)
            --(axis cs:1,0.110392443835735)
            --cycle;
            
            \path [fill=TUMAccentGreen, fill opacity=0.3]
            (axis cs:1,0.300433039665222)
            --(axis cs:1,0.217270523309708)
            --(axis cs:10,0.029975451529026)
            --(axis cs:100,0.0137826036661863)
            --(axis cs:1030,2.69307111011585e-05)
            --(axis cs:1030,3.39279649779201e-05)
            --(axis cs:1030,3.39279649779201e-05)
            --(axis cs:100,0.0635760053992271)
            --(axis cs:10,0.122605122625828)
            --(axis cs:1,0.300433039665222)
            --cycle;
            
            \path [fill=TUMDarkGray, fill opacity=0.3]
            (axis cs:1,0.0162415113300085)
            --(axis cs:1,0.00787685066461563)
            --(axis cs:10,0.0011666618520394)
            --(axis cs:100,0.000416445749578997)
            --(axis cs:1030,2.69307111011585e-05)
            --(axis cs:1030,3.39279649779201e-05)
            --(axis cs:1030,3.39279649779201e-05)
            --(axis cs:100,0.00120243022684008)
            --(axis cs:10,0.00445352960377932)
            --(axis cs:1,0.0162415113300085)
            --cycle;
            
            \addplot [very thick, TUMBlue, dotted]
            table {%
            1 0.970893800258636
            10 0.971157640218735
            100 0.970987439155579
            1030 0.971123987436295
            };
            \addplot [very thick, TUMAccentOrange, loosely dashed]
            table {%
            1 0.0735484529286623
            10 0.0909464824944735
            100 0.0809425700455904
            1030 0.0753381453454494
            };
            \addplot [very thick, TUMAccentGreen, dashdotted]
            table {%
            1 0.254467599093914
            10 0.076106196269393
            100 0.0343588937073946
            1030 3.02713924611453e-05
            };
            \addplot [very thick, TUMDarkGray]
            table {%
            1 0.0129273715429008
            10 0.00238468172028661
            100 0.000593619010760449
            1030 3.02713924611453e-05
            };

        \nextgroupplot[ymin=-.01, ymax=1]
            \path [fill=TUMBlue, fill opacity=0.3]
            (axis cs:1,0.978489875793457)
            --(axis cs:1,0.976292133331299)
            --(axis cs:10,0.974530458450317)
            --(axis cs:100,0.975531876087189)
            --(axis cs:768,0.976448774337769)
            --(axis cs:768,0.979049742221832)
            --(axis cs:768,0.979049742221832)
            --(axis cs:100,0.978672683238983)
            --(axis cs:10,0.97836309671402)
            --(axis cs:1,0.978489875793457)
            --cycle;
            
            \path [fill=TUMAccentOrange, fill opacity=0.3]
            (axis cs:1,0.485232621431351)
            --(axis cs:1,0.467283695936203)
            --(axis cs:10,0.467687338590622)
            --(axis cs:100,0.462273567914963)
            --(axis cs:768,0.464079469442368)
            --(axis cs:768,0.494135111570358)
            --(axis cs:768,0.494135111570358)
            --(axis cs:100,0.484870672225952)
            --(axis cs:10,0.482773751020432)
            --(axis cs:1,0.485232621431351)
            --cycle;
            
            \path [fill=TUMAccentGreen, fill opacity=0.3]
            (axis cs:1,0.49892070889473)
            --(axis cs:1,0.479660511016846)
            --(axis cs:10,0.331441134214401)
            --(axis cs:100,0.29341733455658)
            --(axis cs:768,0.265404492616653)
            --(axis cs:768,0.338111042976379)
            --(axis cs:768,0.338111042976379)
            --(axis cs:100,0.329336136579514)
            --(axis cs:10,0.394336879253387)
            --(axis cs:1,0.49892070889473)
            --cycle;
            
            \path [fill=TUMDarkGray, fill opacity=0.3]
            (axis cs:1,0.341389924287796)
            --(axis cs:1,0.271425068378448)
            --(axis cs:10,0.290894746780396)
            --(axis cs:100,0.291389852762222)
            --(axis cs:768,0.265404492616653)
            --(axis cs:768,0.338111042976379)
            --(axis cs:768,0.338111042976379)
            --(axis cs:100,0.325631946325302)
            --(axis cs:10,0.356628745794296)
            --(axis cs:1,0.341389924287796)
            --cycle;
            
            \addplot [very thick, TUMBlue, dotted]
            table {%
            1 0.977634418010712
            10 0.977157086133957
            100 0.977373641729355
            768 0.977837258577347
            };
            \addplot [very thick, TUMAccentOrange, loosely dashed]
            table {%
            1 0.478096976876259
            10 0.47428266108036
            100 0.474948781728744
            768 0.477871817350388
            };
            \addplot [very thick, TUMAccentGreen, dashdotted]
            table {%
            1 0.490687200427055
            10 0.363046365976334
            100 0.313851061463356
            768 0.304943886399269
            };
            \addplot [very thick, TUMDarkGray]
            table {%
            1 0.304748892784119
            10 0.323556742072105
            100 0.310805207490921
            768 0.304943889379501
            };

        \nextgroupplot[ymin=-.01, ymax=1]
            \path [fill=TUMBlue, fill opacity=0.3]
            (axis cs:1,0.974865078926086)
            --(axis cs:1,0.972657382488251)
            --(axis cs:10,0.972707331180573)
            --(axis cs:100,0.972871720790863)
            --(axis cs:768,0.972386479377747)
            --(axis cs:768,0.975238263607025)
            --(axis cs:768,0.975238263607025)
            --(axis cs:100,0.974535584449768)
            --(axis cs:10,0.974564492702484)
            --(axis cs:1,0.974865078926086)
            --cycle;
            
            \path [fill=TUMAccentOrange, fill opacity=0.3]
            (axis cs:1,0.103296421468258)
            --(axis cs:1,0.0710046887397766)
            --(axis cs:10,0.0530183687806129)
            --(axis cs:100,0.0463272109627724)
            --(axis cs:768,0.0598243847489357)
            --(axis cs:768,0.112838260829449)
            --(axis cs:768,0.112838260829449)
            --(axis cs:100,0.131321057677269)
            --(axis cs:10,0.116678237915039)
            --(axis cs:1,0.103296421468258)
            --cycle;
            
            \path [fill=TUMAccentGreen, fill opacity=0.3]
            (axis cs:1,0.430793642997742)
            --(axis cs:1,0.360972732305527)
            --(axis cs:10,0.065138153731823)
            --(axis cs:100,0.0323449894785881)
            --(axis cs:768,0.0399945974349976)
            --(axis cs:768,0.0638706460595131)
            --(axis cs:768,0.0638706460595131)
            --(axis cs:100,0.0771550089120865)
            --(axis cs:10,0.117947183549404)
            --(axis cs:1,0.430793642997742)
            --cycle;
            
            \path [fill=TUMDarkGray, fill opacity=0.3]
            (axis cs:1,0.0668349862098694)
            --(axis cs:1,0.0369785279035568)
            --(axis cs:10,0.0562192872166634)
            --(axis cs:100,0.031758327037096)
            --(axis cs:768,0.0399946011602879)
            --(axis cs:768,0.0638706460595131)
            --(axis cs:768,0.0638706460595131)
            --(axis cs:100,0.0772484615445137)
            --(axis cs:10,0.0818392634391785)
            --(axis cs:1,0.0668349862098694)
            --cycle;
            
            \addplot [very thick, TUMBlue, dotted]
            table {%
            1 0.973845708370209
            10 0.973784959316254
            100 0.973809826374054
            768 0.974190872907639
            };
            \addplot [very thick, TUMAccentOrange, loosely dashed]
            table {%
            1 0.0855244427919388
            10 0.0822113148868084
            100 0.0754594754427671
            768 0.0903380356729031
            };
            \addplot [very thick, TUMAccentGreen, dashdotted]
            table {%
            1 0.400088629126549
            10 0.0842975057661533
            100 0.0507550314068794
            768 0.0506364308297634
            };
            \addplot [very thick, TUMDarkGray]
            table {%
            1 0.0532312855124474
            10 0.0696122348308563
            100 0.0488714564591646
            768 0.0506364312022924
            };
    \end{groupplot}

    \path (group c1r2.south east) -- node[below=1.2cm]{\pgfplotslegendfromname{CommonLegend2}} (group c2r2.south west);
\end{tikzpicture}

\end{document}
