# Supplementary material for: Learning Expressive Priors for Generalization and Uncertainty Estimation in Neural Networks
Source: arXiv:2307.07753 source file (2026-03-30)
Supplement: Supplementary file 3 [file cold_posterior_large.tex]

\documentclass{standalone}
\usepackage[ansinew]{inputenc}

\usepackage{../../tikz_include}

\begin{document}

\begin{tikzpicture}
\begin{axis}[
name=boundary,
footnotesize,
width=\textwidth,
height=0.6\textwidth,
log basis x={10},
xlabel={Temperature scaling $\tau$},
xmode=log,
max space between ticks=40pt,
ylabel={Accuracy},
ymin=0, ymax=100,
]
\path [draw=TUMBlue, fill=TUMBlue, opacity=0.2]
(axis cs:1e-15,90.1)
--(axis cs:1e-15,88.78)
--(axis cs:1e-14,88.77)
--(axis cs:1e-13,77.44)
--(axis cs:1e-12,9.96)
--(axis cs:1e-11,9.6)
--(axis cs:1e-10,10.21)
--(axis cs:1e-09,9.7)
--(axis cs:1e-08,10.03)
--(axis cs:1e-08,10.32)
--(axis cs:1e-08,10.32)
--(axis cs:1e-09,10.35)
--(axis cs:1e-10,10.37)
--(axis cs:1e-11,10.32)
--(axis cs:1e-12,10.79)
--(axis cs:1e-13,84.42)
--(axis cs:1e-14,90.12)
--(axis cs:1e-15,90.1)
--cycle;
\path [draw=TUMBlue, fill=TUMBlue, opacity=0.2]
(axis cs:1e-15,90.77)
--(axis cs:1e-15,88.31)
--(axis cs:1e-14,88.31)
--(axis cs:1e-13,88.31)
--(axis cs:1e-12,88.28)
--(axis cs:1e-11,10.2)
--(axis cs:1e-10,9.99)
--(axis cs:1e-09,10)
--(axis cs:1e-08,10)
--(axis cs:1e-08,10.02)
--(axis cs:1e-08,10.02)
--(axis cs:1e-09,10)
--(axis cs:1e-10,10)
--(axis cs:1e-11,36.96)
--(axis cs:1e-12,90.73)
--(axis cs:1e-13,90.78)
--(axis cs:1e-14,90.77)
--(axis cs:1e-15,90.77)
--cycle;
\path [draw=TUMAccentOrange, fill=TUMAccentOrange, opacity=0.2]
(axis cs:1e-15,85.39)
--(axis cs:1e-15,10.07)
--(axis cs:1e-14,9.73)
--(axis cs:1e-13,10)
--(axis cs:1e-12,10)
--(axis cs:1e-11,10)
--(axis cs:1e-10,10)
--(axis cs:1e-09,10)
--(axis cs:1e-08,10)
--(axis cs:1e-08,10)
--(axis cs:1e-08,10)
--(axis cs:1e-09,10)
--(axis cs:1e-10,10)
--(axis cs:1e-11,10)
--(axis cs:1e-12,10)
--(axis cs:1e-13,10)
--(axis cs:1e-14,14.56)
--(axis cs:1e-15,85.39)
--cycle;
\path [draw=TUMAccentOrange, fill=TUMAccentOrange, opacity=0.2]
(axis cs:1e-15,87.93)
--(axis cs:1e-15,84.87)
--(axis cs:1e-14,84.87)
--(axis cs:1e-13,84.87)
--(axis cs:1e-12,85.53)
--(axis cs:1e-11,84.83)
--(axis cs:1e-10,84.8)
--(axis cs:1e-09,10)
--(axis cs:1e-08,10)
--(axis cs:1e-08,10.09)
--(axis cs:1e-08,10.09)
--(axis cs:1e-09,87.07)
--(axis cs:1e-10,87.88)
--(axis cs:1e-11,87.93)
--(axis cs:1e-12,87.57)
--(axis cs:1e-13,87.93)
--(axis cs:1e-14,87.93)
--(axis cs:1e-15,87.93)
--cycle;
\addplot [very thick, TUMAccentOrange, dotted]
table {%
1e-15 35.31
1e-14 11.43
1e-13 10
1e-12 10
1e-11 10
1e-10 10
1e-09 10
1e-08 10
};
\label{pgfplots:cold_posterior_iso_5}
\addplot [very thick, TUMAccentOrange, dotted, mark=*]
table {%
1e-15 86.55
1e-14 86.55
1e-13 86.55
1e-12 86.55
1e-11 86.54
1e-10 86.52
1e-09 35.69
1e-08 10.03
};
\label{pgfplots:cold_posterior_iso_3}
\addplot [very thick, TUMBlue]
table {%
1e-15 89.3666666666667
1e-14 89.37
1e-13 81.8233333333333
1e-12 10.26
1e-11 10.0433333333333
1e-10 10.2633333333333
1e-09 10.0066666666667
1e-08 10.13
};
\label{pgfplots:cold_posterior_learned_5}
\addplot [very thick, TUMBlue, mark=*]
table {%
1e-15 89.3933333333333
1e-14 89.3933333333333
1e-13 89.3966666666667
1e-12 89.3866666666667
1e-11 19.81
1e-10 9.99666666666667
1e-09 10
1e-08 10.0066666666667
};
\label{pgfplots:cold_posterior_learned_3}

\end{axis}
\node[draw,fill=white,inner sep=2pt, below=1cm] at (boundary.south) {\small
    \begin{tabular}{ccl}
    $\gamma = 10^{-3}$ & $\gamma = 10^{-5}$ \\
    \ref{pgfplots:cold_posterior_iso_3} & \ref{pgfplots:cold_posterior_iso_5} & isotropic\\
    \ref{pgfplots:cold_posterior_learned_3} & \ref{pgfplots:cold_posterior_learned_5} & learned
    \end{tabular}};
\end{tikzpicture}

\end{document}
