# Supplementary material for: Learning Expressive Priors for Generalization and Uncertainty Estimation in Neural Networks
Source: arXiv:2307.07753 source file (2026-03-30)
Supplement: Supplementary file 4 [file cold_posterior_small.tex]

\documentclass{standalone}
\usepackage[ansinew]{inputenc}

\usepackage{../../tikz_include}

\begin{document}

\begin{tikzpicture}
\begin{axis}[
name=boundary,
footnotesize,
width=\textwidth,
height=0.6\textwidth,
log basis x={10},
xlabel={Temperature scaling $\tau$},
xmode=log,
max space between ticks=40pt,
ylabel={Accuracy},
ymin=0, ymax=100,
]
\path [draw=TUMBlue, fill=TUMBlue, opacity=0.2]
(axis cs:1e-09,94.4730461956522)
--(axis cs:1e-09,94.4057554347826)
--(axis cs:1e-08,94.4049945652174)
--(axis cs:1e-07,94.4026059782609)
--(axis cs:1e-06,94.4033695652174)
--(axis cs:1e-05,94.401847826087)
--(axis cs:0.0001,94.3995434782609)
--(axis cs:0.001,94.4040217391305)
--(axis cs:0.01,94.4179347826087)
--(axis cs:0.1,94.3010679347826)
--(axis cs:0.3,92.5034782608696)
--(axis cs:1,63.6435923913044)
--(axis cs:1,73.5165597826087)
--(axis cs:1,73.5165597826087)
--(axis cs:0.3,93.1888179347826)
--(axis cs:0.1,94.3600271739131)
--(axis cs:0.01,94.4880652173913)
--(axis cs:0.001,94.4719565217391)
--(axis cs:0.0001,94.4716331521739)
--(axis cs:1e-05,94.4690244565217)
--(axis cs:1e-06,94.4699130434783)
--(axis cs:1e-07,94.4684809782609)
--(axis cs:1e-08,94.472285326087)
--(axis cs:1e-09,94.4730461956522)
--cycle;
\path [draw=TUMBlue, fill=TUMBlue, opacity=0.2]
(axis cs:1e-09,94.4257690217391)
--(axis cs:1e-09,94.3645516304347)
--(axis cs:1e-08,94.3651086956522)
--(axis cs:1e-07,94.3640163043478)
--(axis cs:1e-06,94.36325)
--(axis cs:1e-05,94.3651059782609)
--(axis cs:0.0001,94.3604320652174)
--(axis cs:0.001,94.3659782608696)
--(axis cs:0.01,94.3749782608696)
--(axis cs:0.1,94.2519565217391)
--(axis cs:0.3,92.3869510869565)
--(axis cs:1,64.0437798913044)
--(axis cs:1,73.6619701086957)
--(axis cs:1,73.6619701086957)
--(axis cs:0.3,93.1041114130435)
--(axis cs:0.1,94.3155625)
--(axis cs:0.01,94.4333858695652)
--(axis cs:0.001,94.4262065217391)
--(axis cs:0.0001,94.4204402173913)
--(axis cs:1e-05,94.4253288043478)
--(axis cs:1e-06,94.4229347826087)
--(axis cs:1e-07,94.4220733695652)
--(axis cs:1e-08,94.4232663043478)
--(axis cs:1e-09,94.4257690217391)
--cycle;
\path [draw=TUMBlue, fill=TUMBlue, opacity=0.2]
(axis cs:1e-09,94.4223131868132)
--(axis cs:1e-09,94.3625274725275)
--(axis cs:1e-08,94.3657087912088)
--(axis cs:1e-07,94.3627119565217)
--(axis cs:1e-06,94.3629347826087)
--(axis cs:1e-05,94.3597798913043)
--(axis cs:0.0001,94.3629266304348)
--(axis cs:0.001,94.3599918478261)
--(axis cs:0.01,94.3733668478261)
--(axis cs:0.1,94.2356521739131)
--(axis cs:0.3,92.4872994505494)
--(axis cs:1,64.073402173913)
--(axis cs:1,73.7797173913043)
--(axis cs:1,73.7797173913043)
--(axis cs:0.3,93.0761401098901)
--(axis cs:0.1,94.3001141304348)
--(axis cs:0.01,94.4314157608696)
--(axis cs:0.001,94.417722826087)
--(axis cs:0.0001,94.4212010869565)
--(axis cs:1e-05,94.4182663043478)
--(axis cs:1e-06,94.4196875)
--(axis cs:1e-07,94.4213233695652)
--(axis cs:1e-08,94.4220934065934)
--(axis cs:1e-09,94.4223131868132)
--cycle;
\path [draw=TUMAccentOrange, dotted, fill=TUMAccentOrange, dotted, opacity=0.2]
(axis cs:1e-09,91.4422079207921)
--(axis cs:1e-09,84.3317722772277)
--(axis cs:1e-08,82.2899034653465)
--(axis cs:1e-07,78.8668737623762)
--(axis cs:1e-06,78.5922797029703)
--(axis cs:1e-05,77.2138094059406)
--(axis cs:0.0001,77.3369925742574)
--(axis cs:0.001,76.8623762376237)
--(axis cs:0.01,76.2221930693069)
--(axis cs:0.1,75.2677178217822)
--(axis cs:0.3,68.2386633663366)
--(axis cs:1,43.2894975247525)
--(axis cs:1,55.6192004950495)
--(axis cs:1,55.6192004950495)
--(axis cs:0.3,78.5704752475248)
--(axis cs:0.1,84.7154084158416)
--(axis cs:0.01,86.105004950495)
--(axis cs:0.001,86.3148366336633)
--(axis cs:0.0001,86.4148292079208)
--(axis cs:1e-05,86.7231188118812)
--(axis cs:1e-06,87.3487351485148)
--(axis cs:1e-07,88.1179603960396)
--(axis cs:1e-08,89.9049925742574)
--(axis cs:1e-09,91.4422079207921)
--cycle;
\path [draw=TUMAccentOrange, dotted, fill=TUMAccentOrange, dotted, opacity=0.2]
(axis cs:1e-09,95.1996994949495)
--(axis cs:1e-09,94.8928661616162)
--(axis cs:1e-08,90.7155732323232)
--(axis cs:1e-07,85.5477247474748)
--(axis cs:1e-06,82.5818484848485)
--(axis cs:1e-05,78.9540675)
--(axis cs:0.0001,72.813625)
--(axis cs:0.001,71.450975)
--(axis cs:0.01,70.4267054455446)
--(axis cs:0.1,68.5627400990099)
--(axis cs:0.3,62.6555681818182)
--(axis cs:1,39.1733910891089)
--(axis cs:1,50.7825198019802)
--(axis cs:1,50.7825198019802)
--(axis cs:0.3,74.3323939393939)
--(axis cs:0.1,79.2065272277228)
--(axis cs:0.01,80.9370198019802)
--(axis cs:0.001,82.379475)
--(axis cs:0.0001,82.94416)
--(axis cs:1e-05,87.7429225)
--(axis cs:1e-06,90.4418383838384)
--(axis cs:1e-07,91.917702020202)
--(axis cs:1e-08,94.6179595959596)
--(axis cs:1e-09,95.1996994949495)
--cycle;
\path [draw=TUMAccentOrange, dotted, fill=TUMAccentOrange, dotted, opacity=0.2]
(axis cs:1e-09,95.2257601010101)
--(axis cs:1e-09,95.1757575757576)
--(axis cs:1e-08,95.1785858585859)
--(axis cs:1e-07,95.150404040404)
--(axis cs:1e-06,93.6342373737374)
--(axis cs:1e-05,90.4725631313131)
--(axis cs:0.0001,88.4959040404041)
--(axis cs:0.001,86.6577676767677)
--(axis cs:0.01,83.3282095959596)
--(axis cs:0.1,79.5617676767677)
--(axis cs:0.3,72.0609166666667)
--(axis cs:1,43.8232954545455)
--(axis cs:1,56.6672777777778)
--(axis cs:1,56.6672777777778)
--(axis cs:0.3,81.1660202020202)
--(axis cs:0.1,87.6034419191919)
--(axis cs:0.01,89.9588333333333)
--(axis cs:0.001,92.2966641414141)
--(axis cs:0.0001,93.2747727272727)
--(axis cs:1e-05,94.1031944444444)
--(axis cs:1e-06,95.0157777777778)
--(axis cs:1e-07,95.2083863636364)
--(axis cs:1e-08,95.2258737373737)
--(axis cs:1e-09,95.2257601010101)
--cycle;
\path [draw=TUMAccentGreen, loosely dashed, fill=TUMAccentGreen, loosely dashed, opacity=0.2]
(axis cs:1e-09,91.8694615384615)
--(axis cs:1e-09,75.9917884615385)
--(axis cs:1e-08,75.3292307692308)
--(axis cs:1e-07,74.337625)
--(axis cs:1e-06,73.6776442307692)
--(axis cs:1e-05,73.505)
--(axis cs:0.0001,73.7437884615385)
--(axis cs:0.001,73.2862403846154)
--(axis cs:0.01,71.6508942307692)
--(axis cs:0.1,70.3256153846154)
--(axis cs:0.3,55.1269519230769)
--(axis cs:1,15.7692115384615)
--(axis cs:1,20.8703269230769)
--(axis cs:1,20.8703269230769)
--(axis cs:0.3,74.2320961538462)
--(axis cs:0.1,88.2959326923077)
--(axis cs:0.01,89.1400192307692)
--(axis cs:0.001,89.5157788461538)
--(axis cs:0.0001,89.6608653846154)
--(axis cs:1e-05,89.8945384615385)
--(axis cs:1e-06,90.1220384615385)
--(axis cs:1e-07,90.7751538461538)
--(axis cs:1e-08,90.2712980769231)
--(axis cs:1e-09,91.8694615384615)
--cycle;
\path [draw=TUMAccentGreen, loosely dashed, fill=TUMAccentGreen, loosely dashed, opacity=0.2]
(axis cs:1e-09,95.2050096153846)
--(axis cs:1e-09,94.99575)
--(axis cs:1e-08,85.4929038461539)
--(axis cs:1e-07,72.3305)
--(axis cs:1e-06,66.7356730769231)
--(axis cs:1e-05,63.43175)
--(axis cs:0.0001,63.2595576923077)
--(axis cs:0.001,63.1035096153846)
--(axis cs:0.01,63.6133461538461)
--(axis cs:0.1,63.0602019230769)
--(axis cs:0.3,45.1547596153846)
--(axis cs:1,12.637875)
--(axis cs:1,15.7209134615385)
--(axis cs:1,15.7209134615385)
--(axis cs:0.3,65.0158076923077)
--(axis cs:0.1,83.4797019230769)
--(axis cs:0.01,84.7387115384615)
--(axis cs:0.001,84.5898365384615)
--(axis cs:0.0001,84.2302980769231)
--(axis cs:1e-05,84.2529230769231)
--(axis cs:1e-06,85.8731826923077)
--(axis cs:1e-07,89.929375)
--(axis cs:1e-08,94.5071538461538)
--(axis cs:1e-09,95.2050096153846)
--cycle;
\path [draw=TUMAccentGreen, loosely dashed, fill=TUMAccentGreen, loosely dashed, opacity=0.2]
(axis cs:1e-09,95.2338557692308)
--(axis cs:1e-09,95.1469134615385)
--(axis cs:1e-08,95.1457692307692)
--(axis cs:1e-07,94.8326730769231)
--(axis cs:1e-06,83.5637692307692)
--(axis cs:1e-05,75.9562692307692)
--(axis cs:0.0001,75.2325865384615)
--(axis cs:0.001,71.6749423076923)
--(axis cs:0.01,70.8860192307693)
--(axis cs:0.1,69.6582788461538)
--(axis cs:0.3,57.4634807692308)
--(axis cs:1,14.7155961538462)
--(axis cs:1,19.6518653846154)
--(axis cs:1,19.6518653846154)
--(axis cs:0.3,76.6077307692308)
--(axis cs:0.1,90.5640480769231)
--(axis cs:0.01,91.5362115384615)
--(axis cs:0.001,91.9795961538461)
--(axis cs:0.0001,92.6337115384615)
--(axis cs:1e-05,94.0239903846154)
--(axis cs:1e-06,95.030125)
--(axis cs:1e-07,95.2157788461539)
--(axis cs:1e-08,95.2373076923077)
--(axis cs:1e-09,95.2338557692308)
--cycle;
\addplot [very thick, TUMBlue, mark=|]
table {%
9.99999971718069e-10 94.4372863769531
0.000999999465420842 94.4379348754883
0.00999999418854713 94.4517364501953
0.100000001490116 94.3306503295898
0.299999982118607 92.8483657836914
1 68.5803298950195
};
\label{pgfplots:cold_posterior_small_learned_8}
\addplot [very thick, TUMBlue]
table {%
9.99999971718069e-10 94.3940200805664
9.99998883344233e-06 94.3946762084961
9.99999974737875e-05 94.3903274536133
0.00999999418854713 94.4031524658203
0.100000001490116 94.2835845947266
0.299999982118607 92.7732620239258
1 69.0018463134766
};
\label{pgfplots:cold_posterior_small_learned_5}
\addplot [very thick, TUMBlue, mark=*]
table {%
9.99999971718069e-10 94.3925247192383
0.000999999465420842 94.3893508911133
0.00999999418854713 94.4010848999023
0.100000001490116 94.2701110839844
0.299999982118607 92.7926406860352
1 69.0880432128906
};
\label{pgfplots:cold_posterior_small_learned_3}
\addplot [very thick, TUMAccentOrange, dotted, mark=|]
table {%
9.99999971718069e-10 88.0781173706055
9.9999777347648e-09 86.2591094970703
9.9999887481772e-08 83.4696044921875
9.99998860606865e-07 83.029899597168
9.99998883344233e-06 82.2221755981445
9.99999974737875e-05 82.0034637451172
0.000999999465420842 81.7080230712891
0.00999999418854713 81.3465347290039
0.100000001490116 80.1801986694336
0.299999982118607 73.6076202392578
1 49.6616821289062
};
\label{pgfplots:cold_posterior_small_iso_8}
\addplot [very thick, TUMAccentOrange, dotted]
table {%
9.99999971718069e-10 95.0874710083008
9.9999777347648e-09 93.0270690917969
9.9999887481772e-08 89.0841445922852
9.99998860606865e-07 86.8150482177734
9.99998883344233e-06 83.7592010498047
9.99999974737875e-05 78.3619003295898
0.000999999465420842 77.3093032836914
0.00999999418854713 76.0009918212891
0.100000001490116 73.8769302368164
0.299999982118607 68.5429306030273
1 44.5184173583984
};
\label{pgfplots:cold_posterior_small_iso_5}
\addplot [very thick, TUMAccentOrange, dotted, mark=*]
table {%
9.99999971718069e-10 95.2022247314453
9.9999777347648e-09 95.2021179199219
9.9999887481772e-08 95.1786880493164
9.99998860606865e-07 94.4511108398438
9.99998883344233e-06 92.5080795288086
9.99999974737875e-05 91.1372756958008
0.000999999465420842 89.7161636352539
0.00999999418854713 86.9089889526367
0.100000001490116 83.8316192626953
0.299999982118607 76.5757598876953
1 50.3021202087402
};
\label{pgfplots:cold_posterior_small_iso_3}
\addplot [very thick, TUMAccentGreen, loosely dashed, mark=|]
table {%
9.99999971718069e-10 84.7576904296875
9.9999777347648e-09 83.5638427734375
9.9999887481772e-08 83.1165390014648
9.99998860606865e-07 82.6365356445312
9.99998883344233e-06 82.2303848266602
9.99999974737875e-05 81.9961547851562
0.000999999465420842 81.982307434082
0.00999999418854713 80.903076171875
0.100000001490116 79.5192337036133
0.299999982118607 65.2061538696289
1 18.3103847503662
};
\label{pgfplots:cold_posterior_small_0_8}
\addplot [very thick, TUMAccentGreen, loosely dashed]
table {%
9.99999971718069e-10 95.114616394043
9.9999777347648e-09 90.9373092651367
9.9999887481772e-08 82.0988464355469
9.99998860606865e-07 76.6053848266602
9.99998883344233e-06 74.7415390014648
9.99999974737875e-05 74.2584609985352
0.000999999465420842 73.8057708740234
0.00999999418854713 74.7180786132812
0.100000001490116 73.7850036621094
0.299999982118607 54.7165374755859
1 14.0569229125977
};
\label{pgfplots:cold_posterior_small_0_5}
\addplot [very thick, TUMAccentGreen, loosely dashed, mark=*]
table {%
9.99999971718069e-10 95.1903839111328
9.9999777347648e-09 95.1930770874023
9.9999887481772e-08 95.0707702636719
9.99998860606865e-07 90.4026947021484
9.99998883344233e-06 86.4796142578125
9.99999974737875e-05 84.8807678222656
0.000999999465420842 83.0853881835938
0.00999999418854713 82.5784606933594
0.100000001490116 81.4203872680664
0.299999982118607 67.1846160888672
1 17.0653839111328
};
\label{pgfplots:cold_posterior_small_0_3}

\end{axis}
\node[draw,fill=white,inner sep=2pt, below=1cm] at (boundary.south) {\small
    \begin{tabular}{cccl}
    $\gamma = 10^{-3}$ & $\gamma = 10^{-5}$ & $\gamma = 10^{-8}$ \\
    \ref{pgfplots:cold_posterior_small_0_3} & \ref{pgfplots:cold_posterior_small_0_5} & \ref{pgfplots:cold_posterior_small_0_8} & zero mean \& isotropic\\
    \ref{pgfplots:cold_posterior_small_iso_3} & \ref{pgfplots:cold_posterior_small_iso_5} & \ref{pgfplots:cold_posterior_small_iso_8} & isotropic\\
    \ref{pgfplots:cold_posterior_small_learned_3} & \ref{pgfplots:cold_posterior_small_learned_5} & \ref{pgfplots:cold_posterior_small_learned_8} & learned
    \end{tabular}};
\end{tikzpicture}

\end{document}
