# Supplementary material for: Learning Expressive Priors for Generalization and Uncertainty Estimation in Neural Networks
Source: arXiv:2307.07753 source file (2026-03-30)
Supplement: Supplementary file 5 [file results_small_data.tex]

\documentclass{standalone}
\usepackage[ansinew]{inputenc}

\usepackage{../../tikz_include}

\begin{document}

\begin{tikzpicture}
\begin{groupplot}[
footnotesize,
width=0.25\textwidth,
group style={
group size=5 by 8, 
y descriptions at=edge left, 
x descriptions at=edge bottom,
horizontal sep=.25cm,
vertical sep=.25cm
},
xlabel={num samples},
xmin=0.650699258757847, xmax=8298.76464022464,
xmode=log,
log basis x={10},
ylabel={accuracy},
ymin=0, ymax=100,
]
\nextgroupplot[
title={$\tau = 0.001$},
legend to name={LegendSmallData},
legend style={legend columns=3}, 
]
\addplot [very thick, TUMAccentGreen, loosely dashed]
table {%
1 9.86999988555908
2 10.6099996566772
5 10
10 9.98999977111816
20 9.78999996185303
50 9.64000034332275
100 10.0200004577637
200 11.1700000762939
500 78.379997253418
1000 81.8099975585938
2000 93.8399963378906
5000 95.3300018310547
5400 95.2900009155273
};
\addlegendentry{zero mean \& isotropic}
\addplot [very thick, TUMAccentOrange, dotted]
table {%
1 10.0299997329712
2 9.98999977111816
5 10.1099996566772
10 9.97999954223633
20 9.98999977111816
50 9.94999980926514
100 10.5
200 11.5799999237061
500 24.7099990844727
1000 92.3899993896484
2000 94.0599975585938
5000 94.9400024414062
5400 95.2699966430664
};
\addlegendentry{isotropic}
\addplot [very thick, TUMBlue]
table {%
1 10
2 9.82999992370605
5 9.97999954223633
10 11.8400001525879
20 16.3700008392334
50 51.7200012207031
100 78.2600021362305
200 87.8899993896484
500 91.3899993896484
1000 92.4199981689453
2000 93.1600036621094
5000 94.3300018310547
5400 94.6100006103516
};
\addlegendentry{learned}
\nextgroupplot[
title={$\tau = 10^{-5}$},
]
\addplot [very thick, TUMBlue]
table {%
1 12.1000003814697
2 36.2299995422363
5 35.7299995422363
10 53.1199989318848
20 61.9599990844727
50 83.6800003051758
100 87.1900024414062
200 89.2300033569336
500 91.5400009155273
1000 92.4499969482422
2000 93.25
5000 94.3499984741211
5400 94.5999984741211
};
\addplot [very thick, TUMAccentOrange, dotted]
table {%
1 10.0100002288818
2 10.0200004577637
5 10.0200004577637
20 10.4200000762939
50 21.9699993133545
100 58.1399993896484
200 70.8199996948242
500 90.5
1000 92.9300003051758
2000 94.0500030517578
5000 94.9700012207031
5400 95.2799987792969
};
\addplot [very thick, TUMAccentGreen, loosely dashed]
table {%
1 9.92000007629395
2 9.22000026702881
5 10
10 9.92000007629395
20 10.2200002670288
50 10.1499996185303
100 64.0500030517578
200 87.5699996948242
500 91.8399963378906
1000 93.2600021362305
2000 93.8499984741211
5000 95.3099975585938
5400 95.2600021362305
};
\nextgroupplot[
title={$\tau = 10^{-7}$},
]
\addplot [very thick, TUMBlue]
table {%
1 23.1499996185303
2 40.7400016784668
5 41.0900001525879
10 53.6199989318848
20 62.0099983215332
50 83.6500015258789
100 87.25
200 89.2099990844727
500 91.5299987792969
1000 92.4499969482422
2000 93.25
5000 94.3499984741211
5400 94.6100006103516
};
\addplot [very thick, TUMAccentOrange, dotted]
table {%
1 17.7900009155273
2 42.1599998474121
5 61.1599998474121
10 26.6100006103516
20 56.4799995422363
50 85.0800018310547
100 88.370002746582
200 89.6500015258789
500 92.0500030517578
1000 92.9899978637695
2000 94.0500030517578
5000 94.9700012207031
5400 95.2900009155273
};
\addplot [very thick, TUMAccentGreen, loosely dashed]
table {%
1 23.6200008392334
2 25.8199996948242
5 12.9899997711182
10 19.6399993896484
20 53.3400001525879
50 85.1500015258789
100 87.6800003051758
200 90.6600036621094
500 92.3300018310547
1000 93.3499984741211
2000 93.8600006103516
5000 95.3000030517578
5400 95.2600021362305
};
\nextgroupplot[
title={$\tau = 10^{-9}$},
]
\addplot [very thick, TUMBlue]
table {%
1 23.0699996948242
2 40.8300018310547
5 41.0800018310547
10 53.6199989318848
20 61.9900016784668
50 83.6500015258789
100 87.2600021362305
200 89.2099990844727
500 91.5299987792969
1000 92.4599990844727
2000 93.25
5000 94.3499984741211
5400 94.6100006103516
};
\addplot [very thick, TUMAccentOrange, dotted]
table {%
1 19.7299995422363
2 41.8699989318848
5 69.4899978637695
10 76.129997253418
20 78.870002746582
50 85.370002746582
100 88.370002746582
200 89.8300018310547
500 92.0299987792969
1000 92.9899978637695
2000 94.0500030517578
5000 94.9700012207031
5400 95.2900009155273
};
\addplot [very thick, TUMAccentGreen, loosely dashed]
table {%
1 34.9000015258789
2 51.4500007629395
5 64.8300018310547
10 76.6500015258789
20 81.1500015258789
50 85.5899963378906
100 87.75
200 90.6900024414062
500 92.3099975585938
1000 93.3600006103516
2000 93.8600006103516
5000 95.3000030517578
5400 95.2600021362305
};
\nextgroupplot[
title={$10^{-11}$},
ylabel style={rotate=-90},
ytick pos=right,%
ylabel={$\gamma = 0.01$},%
]
\addplot [very thick, TUMBlue]
table {%
1 23.0499992370605
2 40.8199996948242
5 41.0699996948242
10 53.6199989318848
20 62
50 83.6500015258789
100 87.2600021362305
200 89.2099990844727
500 91.5299987792969
1000 92.4599990844727
2000 93.25
5000 94.3499984741211
5400 94.6100006103516
};
\addplot [very thick, TUMAccentOrange, dotted]
table {%
1 19.7299995422363
2 41.8400001525879
5 69.4599990844727
10 76.1800003051758
20 78.8399963378906
50 85.379997253418
100 88.3600006103516
200 89.8300018310547
500 92.0299987792969
1000 92.9899978637695
2000 94.0500030517578
5000 94.9700012207031
5400 95.2900009155273
};
\addplot [very thick, TUMAccentGreen, loosely dashed]
table {%
1 34.810001373291
2 51.4099998474121
5 65.4899978637695
10 77.1699981689453
20 81.2300033569336
50 85.5999984741211
100 87.7399978637695
200 90.6900024414062
500 92.3099975585938
1000 93.3600006103516
2000 93.8600006103516
5000 95.3000030517578
5400 95.2600021362305
};
\nextgroupplot
\addplot [very thick, TUMBlue]
table {%
1 9.97000026702881
2 9.90999984741211
5 9.9399995803833
10 11.5500001907349
20 21.5499992370605
50 51.6300010681152
100 78.3499984741211
200 87.6800003051758
500 91.2200012207031
1000 92.2099990844727
2000 93.4199981689453
5000 94.5299987792969
5400 94.379997253418
};
\addplot [very thick, TUMAccentOrange, dotted]
table {%
1 10.1700000762939
2 10
5 10.0600004196167
10 10.0600004196167
20 9.98999977111816
50 10.0100002288818
100 9.64000034332275
200 11.7399997711182
500 15.6899995803833
1000 83.5999984741211
2000 90.9800033569336
5000 94.8499984741211
5400 95.1600036621094
};
\addplot [very thick, TUMAccentGreen, loosely dashed]
table {%
1 10.2700004577637
2 9.9399995803833
5 9.98999977111816
10 10.0100002288818
20 10.039999961853
50 10.0500001907349
100 9.9399995803833
200 10.2200002670288
500 15.2399997711182
1000 92.4499969482422
2000 94.0800018310547
5000 94.5199966430664
5400 94.9899978637695
};
\nextgroupplot
\addplot [very thick, TUMBlue]
table {%
1 10.3299999237061
2 34.0499992370605
5 24.5699996948242
10 61.0999984741211
20 61.4799995422363
50 82.4499969482422
100 87.2200012207031
200 89.5
500 91.5199966430664
1000 92.1100006103516
2000 93.4000015258789
5000 94.4800033569336
5400 94.4000015258789
};
\addplot [very thick, TUMAccentOrange, dotted]
table {%
1 10.1499996185303
2 9.96000003814697
5 9.89999961853027
10 9.65999984741211
20 10.289999961853
50 9.92000007629395
100 20.6800003051758
200 78.3099975585938
500 31.6700000762939
1000 92.8499984741211
2000 93.7799987792969
5000 94.8899993896484
5400 95.1399993896484
};
\addplot [very thick, TUMAccentGreen, loosely dashed]
table {%
1 9.55000019073486
2 10.4700002670288
5 10.0100002288818
10 10
20 10
50 10.460000038147
100 21.1900005340576
200 69.9300003051758
500 34.0699996948242
1000 92.6900024414062
2000 94.2099990844727
5000 94.9000015258789
5400 94.9400024414062
};
\nextgroupplot
\addplot [very thick, TUMBlue]
table {%
1 19.3600006103516
2 47.5999984741211
5 39.060001373291
10 61.7900009155273
20 61.7000007629395
50 82.4899978637695
100 87.3000030517578
200 89.5
500 91.5299987792969
1000 92.120002746582
2000 93.4199981689453
5000 94.4899978637695
5400 94.4000015258789
};
\addplot [very thick, TUMAccentOrange, dotted]
table {%
1 9.72999954223633
2 9.90999984741211
5 10.710000038147
10 10.0200004577637
20 10.1599998474121
50 65.8199996948242
100 56.7099990844727
200 89.3199996948242
500 91.0699996948242
1000 93.0100021362305
2000 93.9700012207031
5000 94.8899993896484
5400 95.2600021362305
};
\addplot [very thick, TUMAccentGreen, loosely dashed]
table {%
1 10.1199998855591
2 10.8800001144409
5 10
10 10.3000001907349
20 10.1199998855591
50 79.2699966430664
100 86.4599990844727
200 89.4800033569336
500 62.2799987792969
1000 93.0100021362305
2000 94.1800003051758
5000 95.0599975585938
5400 94.9599990844727
};
\nextgroupplot
\addplot [very thick, TUMBlue]
table {%
1 31.4899997711182
2 47.7000007629395
5 38.9900016784668
10 61.75
20 61.7000007629395
50 82.4800033569336
100 87.3099975585938
200 89.5
500 91.5199966430664
1000 92.120002746582
2000 93.4199981689453
5000 94.4899978637695
5400 94.4000015258789
};
\addplot [very thick, TUMAccentOrange, dotted]
table {%
1 16.6399993896484
2 38.1699981689453
5 17.7999992370605
10 38.689998626709
20 78.3499984741211
50 85.8300018310547
100 87.8000030517578
200 89.8199996948242
500 92.0400009155273
1000 93.0599975585938
2000 93.9599990844727
5000 94.879997253418
5400 95.2900009155273
};
\addplot [very thick, TUMAccentGreen, loosely dashed]
table {%
1 20.6599998474121
2 44.4799995422363
5 12.6800003051758
10 68.9499969482422
20 77.5400009155273
50 85.8899993896484
100 87.8899993896484
200 90.7600021362305
500 92.3399963378906
1000 93.0299987792969
2000 94.1999969482422
5000 95.0699996948242
5400 94.9499969482422
};
\nextgroupplot[
ylabel style={rotate=-90},
ytick pos=right,%
ylabel={$\gamma = 0.001$},%
]
\addplot [very thick, TUMBlue]
table {%
1 31.3199996948242
2 47.7000007629395
5 39.0099983215332
10 61.75
20 61.6800003051758
50 82.4800033569336
100 87.3099975585938
200 89.5
500 91.5199966430664
1000 92.120002746582
2000 93.4199981689453
5000 94.4899978637695
5400 94.4000015258789
};
\addplot [very thick, TUMAccentOrange, dotted]
table {%
1 19.1299991607666
2 42.060001373291
5 67.7099990844727
10 73.5400009155273
20 80.3199996948242
50 85.7399978637695
100 88.3399963378906
200 89.8300018310547
500 92.0199966430664
1000 93.0599975585938
2000 93.9499969482422
5000 94.879997253418
5400 95.2900009155273
};
\addplot [very thick, TUMAccentGreen, loosely dashed]
table {%
1 29.2600002288818
2 44.4799995422363
5 65.9100036621094
10 74.7099990844727
20 80.9899978637695
50 85.9400024414062
100 87.9100036621094
200 90.75
500 92.3499984741211
1000 93.0199966430664
2000 94.1999969482422
5000 95.0699996948242
5400 94.9499969482422
};
\nextgroupplot
\addplot [very thick, TUMBlue]
table {%
1 10.6000003814697
2 9.97999954223633
5 10.210000038147
10 10
20 10.039999961853
50 56.4700012207031
100 76.129997253418
200 86.879997253418
500 91.3300018310547
1000 92.0999984741211
2000 93.4899978637695
5000 94.4499969482422
5400 94.6100006103516
};
\addplot [very thick, TUMAccentOrange, dotted]
table {%
1 9.96000003814697
2 9.5600004196167
5 9.97000026702881
10 10.4499998092651
20 9.5
50 9.75
100 10.3699998855591
200 10.0900001525879
500 14.9300003051758
1000 34.9099998474121
2000 94.3300018310547
5000 95.129997253418
5400 95.0899963378906
};
\addplot [very thick, TUMAccentGreen, loosely dashed]
table {%
1 10.1899995803833
2 10.4399995803833
5 10
10 10.2399997711182
20 9.82999992370605
50 10.0600004196167
100 10.039999961853
200 10.5699996948242
500 82.0400009155273
1000 83.3199996948242
2000 94.2099990844727
5000 94.1699981689453
5400 95.129997253418
};
\nextgroupplot
\addplot [very thick, TUMBlue]
table {%
1 10.3599996566772
2 19.6700000762939
5 31.1499996185303
10 56.810001373291
20 53.1399993896484
50 83.0400009155273
100 87.2699966430664
200 89.879997253418
500 91.3600006103516
1000 92.2900009155273
2000 93.4300003051758
5000 94.4400024414062
5400 94.6100006103516
};
\addplot [very thick, TUMAccentOrange, dotted]
table {%
1 10.039999961853
2 10.3500003814697
5 9.98999977111816
10 9.97000026702881
20 10.3800001144409
50 10.3100004196167
100 10.039999961853
200 20
500 21.5200004577637
1000 44.8699989318848
2000 94.3199996948242
5000 95.1500015258789
5400 95.129997253418
};
\addplot [very thick, TUMAccentGreen, loosely dashed]
table {%
1 10.2200002670288
2 10.2200002670288
5 9.98999977111816
10 10.1000003814697
20 9.76000022888184
50 9.93000030517578
100 11.789999961853
200 51.439998626709
500 92.5
1000 86.0199966430664
2000 94.25
5000 94.5500030517578
5400 95.1399993896484
};
\nextgroupplot
\addplot [very thick, TUMBlue]
table {%
1 19.2000007629395
2 49.3600006103516
5 40.3800010681152
10 59.7700004577637
20 53.8899993896484
50 83.1900024414062
100 87.25
200 89.8499984741211
500 91.3499984741211
1000 92.3000030517578
2000 93.4300003051758
5000 94.4400024414062
5400 94.620002746582
};
\addplot [very thick, TUMAccentOrange, dotted]
table {%
1 9.89000034332275
2 10.4499998092651
5 9.77000045776367
10 10.1999998092651
20 9.82999992370605
50 13.710000038147
100 16.1000003814697
200 42.4099998474121
500 61.8899993896484
1000 90.8600006103516
2000 94.3300018310547
5000 95.1600036621094
5400 95.129997253418
};
\addplot [very thick, TUMAccentGreen, loosely dashed]
table {%
1 10.3000001907349
2 10.289999961853
5 10.0200004577637
10 10.3999996185303
20 10.0799999237061
50 10.4300003051758
100 71.0400009155273
200 71.75
500 92.5100021362305
1000 92.5899963378906
2000 94.25
5000 95.0999984741211
5400 95.1399993896484
};
\nextgroupplot
\addplot [very thick, TUMBlue]
table {%
1 28.0400009155273
2 49.1699981689453
5 40.4700012207031
10 59.7900009155273
20 53.8699989318848
50 83.1999969482422
100 87.2300033569336
200 89.8499984741211
500 91.3499984741211
1000 92.3000030517578
2000 93.4300003051758
5000 94.4400024414062
5400 94.620002746582
};
\addplot [very thick, TUMAccentOrange, dotted]
table {%
1 16.7800006866455
2 10.0200004577637
5 15.5600004196167
10 9.65999984741211
20 12.8599996566772
50 50.4700012207031
100 86.4300003051758
200 89.2300033569336
500 92.1999969482422
1000 93.1800003051758
2000 94.4000015258789
5000 95.1600036621094
5400 95.129997253418
};
\addplot [very thick, TUMAccentGreen, loosely dashed]
table {%
1 10.8299999237061
2 40.8800010681152
5 10
10 10
20 15.1999998092651
50 22.4400005340576
100 87.2300033569336
200 90.5899963378906
500 92.4700012207031
1000 93.0100021362305
2000 94.25
5000 95.1600036621094
5400 95.120002746582
};
\nextgroupplot[
ylabel style={rotate=-90},
ytick pos=right,%
ylabel={$\gamma = 0.0001$},%
]
\addplot [very thick, TUMBlue]
table {%
1 27.75
2 49.1800003051758
5 40.4799995422363
10 59.7799987792969
20 53.8699989318848
50 83.2099990844727
100 87.25
200 89.8499984741211
500 91.3499984741211
1000 92.3000030517578
2000 93.4300003051758
5000 94.4400024414062
5400 94.620002746582
};
\addplot [very thick, TUMAccentOrange, dotted]
table {%
1 31.1299991607666
2 40.810001373291
5 67.8099975585938
10 14.4700002670288
20 76.870002746582
50 85.5899963378906
100 88.4199981689453
200 89.8099975585938
500 92.1800003051758
1000 93.1699981689453
2000 94.370002746582
5000 95.1600036621094
5400 95.129997253418
};
\addplot [very thick, TUMAccentGreen, loosely dashed]
table {%
1 33.1100006103516
2 49.1300010681152
5 9.97999954223633
10 29.6200008392334
20 80.6500015258789
50 84.5100021362305
100 87.3600006103516
200 90.7699966430664
500 92.4700012207031
1000 92.9700012207031
2000 94.25
5000 95.1600036621094
5400 95.129997253418
};
\nextgroupplot
\addplot [very thick, TUMBlue]
table {%
1 9.8100004196167
2 10.1000003814697
5 10.0900001525879
10 11.6400003433228
20 18.1800003051758
50 47.2599983215332
100 82.620002746582
200 86.8600006103516
500 91.4199981689453
1000 92.2699966430664
2000 93.3000030517578
5000 94.4400024414062
5400 94.4100036621094
};
\addplot [very thick, TUMAccentOrange, dotted]
table {%
1 9.93000030517578
2 9.94999980926514
5 10.5699996948242
10 9.78999996185303
20 9.96000003814697
50 10.2799997329712
100 9.80000019073486
200 10.0100002288818
500 89.2099990844727
1000 92.6399993896484
2000 94.0599975585938
5000 95
5400 94.6999969482422
};
\addplot [very thick, TUMAccentGreen, loosely dashed]
table {%
1 9.88000011444092
2 9.81999969482422
5 10
10 10.2600002288818
20 9.97999954223633
50 10.1999998092651
100 9.57999992370605
200 10.4499998092651
500 42.810001373291
1000 92.5800018310547
2000 69.5500030517578
5000 94.0899963378906
5400 94.9400024414062
};
\nextgroupplot
\addplot [very thick, TUMBlue]
table {%
1 10.1899995803833
2 10.1899995803833
5 10.5200004577637
10 46.0999984741211
20 58.8300018310547
50 82.9300003051758
100 86.7799987792969
200 89.1699981689453
500 91.5100021362305
1000 92.2699966430664
2000 93.3000030517578
5000 94.4499969482422
5400 94.4300003051758
};
\addplot [very thick, TUMAccentOrange, dotted]
table {%
1 9.89999961853027
2 10.1099996566772
5 9.85000038146973
10 9.76000022888184
20 9.97999954223633
50 9.86999988555908
100 10.6499996185303
200 87.5699996948242
500 91.5999984741211
1000 92.6500015258789
2000 94.0199966430664
5000 94.9700012207031
5400 95.1900024414062
};
\addplot [very thick, TUMAccentGreen, loosely dashed]
table {%
1 10.0200004577637
2 10.5699996948242
5 10.0299997329712
10 9.71000003814697
20 10.0500001907349
50 9.97999954223633
100 11.9899997711182
200 24.7299995422363
500 54.9000015258789
1000 92.5299987792969
2000 70.4700012207031
5000 94.2099990844727
5400 95.0100021362305
};
\nextgroupplot
\addplot [very thick, TUMBlue]
table {%
1 9.64999961853027
2 17.9400005340576
5 48.0299987792969
10 47.3499984741211
20 58.8199996948242
50 82.8399963378906
100 86.75
200 89.1600036621094
500 91.5100021362305
1000 92.2799987792969
2000 93.3099975585938
5000 94.4499969482422
5400 94.4400024414062
};
\addplot [very thick, TUMAccentOrange, dotted]
table {%
1 9.97000026702881
2 9.47000026702881
5 9.90999984741211
10 9.90999984741211
20 9.69999980926514
50 12.210000038147
100 14.1499996185303
200 88.7799987792969
500 91.870002746582
1000 92.6399993896484
2000 93.9199981689453
5000 94.9700012207031
5400 95.1399993896484
};
\addplot [very thick, TUMAccentGreen, loosely dashed]
table {%
1 10.1300001144409
2 10.0799999237061
5 9.97000026702881
10 10.5
20 10.1400003433228
50 10.6800003051758
100 14.1800003051758
200 44.2000007629395
500 60.4900016784668
1000 92.9199981689453
2000 91.6900024414062
5000 94.6600036621094
5400 95.0999984741211
};
\nextgroupplot
\addplot [very thick, TUMBlue]
table {%
1 10.1000003814697
2 37.9300003051758
5 49.8199996948242
10 47.3499984741211
20 58.7700004577637
50 82.8600006103516
100 86.75
200 89.1699981689453
500 91.5100021362305
1000 92.2799987792969
2000 93.3099975585938
5000 94.4499969482422
5400 94.4400024414062
};
\addplot [very thick, TUMAccentOrange, dotted]
table {%
1 10.1199998855591
2 9.88000011444092
5 9.31999969482422
10 9.76000022888184
20 13.1099996566772
50 54.8300018310547
100 31.3400001525879
200 89.6800003051758
500 92.129997253418
1000 92.7099990844727
2000 93.9800033569336
5000 94.9700012207031
5400 95.2200012207031
};
\addplot [very thick, TUMAccentGreen, loosely dashed]
table {%
1 10.039999961853
2 10.0500001907349
5 10.0100002288818
10 9.89999961853027
20 10.3199996948242
50 14.6199998855591
100 45.7900009155273
200 79.3399963378906
500 91.25
1000 93.1900024414062
2000 94.0199966430664
5000 95
5400 95.129997253418
};
\nextgroupplot[
ylabel style={rotate=-90},
ytick pos=right,%
ylabel={$\gamma = 10^{-5}$},%
]
\addplot [very thick, TUMBlue]
table {%
1 12.5799999237061
2 39.2799987792969
5 49.9799995422363
10 47.3499984741211
20 58.7700004577637
50 82.8600006103516
100 86.75
200 89.1699981689453
500 91.5100021362305
1000 92.2799987792969
2000 93.3099975585938
5000 94.4499969482422
5400 94.4400024414062
};
\addplot [very thick, TUMAccentOrange, dotted]
table {%
1 10
2 10.0500001907349
5 10.6599998474121
10 10.3400001525879
20 76.5999984741211
50 83.6500015258789
100 86.9100036621094
200 89.7200012207031
500 92.1399993896484
1000 92.8199996948242
2000 93.9400024414062
5000 94.9700012207031
5400 95.25
};
\addplot [very thick, TUMAccentGreen, loosely dashed]
table {%
1 10.1599998474121
2 12.960000038147
5 10.1000003814697
10 9.72000026702881
20 13.0200004577637
50 78.6100006103516
100 87.379997253418
200 90.7200012207031
500 92.4000015258789
1000 93.2799987792969
2000 94.129997253418
5000 94.9899978637695
5400 95.129997253418
};
\nextgroupplot
\addplot [very thick, TUMBlue]
table {%
1 9.72000026702881
2 10.1000003814697
5 10.6499996185303
10 11.0699996948242
20 11.4799995422363
50 63.7299995422363
100 79.6399993896484
200 87.5
500 91.0500030517578
1000 92.3600006103516
2000 93.3499984741211
5000 94.5400009155273
5400 94.1800003051758
};
\addplot [very thick, TUMAccentOrange, dotted]
table {%
1 9.72999954223633
2 9.90999984741211
5 9.81999969482422
10 10.0200004577637
20 10
50 9.89000034332275
100 9.25
200 10.1899995803833
500 14.2399997711182
1000 12.2299995422363
2000 92.2600021362305
5000 94.9800033569336
5400 95.2900009155273
};
\addplot [very thick, TUMAccentGreen, loosely dashed]
table {%
1 10.0100002288818
2 10.4099998474121
5 9.71000003814697
10 9.64000034332275
20 10.1300001144409
50 9.65999984741211
100 9.9399995803833
200 10.789999961853
500 85.1900024414062
1000 66.2699966430664
2000 94.1100006103516
5000 88.4300003051758
5400 23.5400009155273
};
\nextgroupplot
\addplot [very thick, TUMBlue]
table {%
1 10.5799999237061
2 10.460000038147
5 11.0200004577637
10 56.9700012207031
20 49.2599983215332
50 81.370002746582
100 87.2200012207031
200 89.2900009155273
500 91.3499984741211
1000 92.3199996948242
2000 93.2799987792969
5000 94.5100021362305
5400 94.1699981689453
};
\addplot [very thick, TUMAccentOrange, dotted]
table {%
1 9.76000022888184
2 10.1199998855591
5 10.0600004196167
10 10.0100002288818
20 10
50 10.3500003814697
100 12.3599996566772
200 42.7900009155273
500 14.8999996185303
1000 11.960000038147
2000 92.2099990844727
5000 95
5400 95.2799987792969
};
\addplot [very thick, TUMAccentGreen, loosely dashed]
table {%
1 10.1899995803833
2 9.67000007629395
5 9.69999980926514
10 10.0699996948242
20 9.80000019073486
50 10.3400001525879
100 13.5500001907349
200 72.9800033569336
500 92.1999969482422
1000 67.0599975585938
2000 94.120002746582
5000 89.25
5400 23.7800006866455
};
\nextgroupplot
\addplot [very thick, TUMBlue]
table {%
1 10.1899995803833
2 10.7399997711182
5 51.0699996948242
10 61.7799987792969
20 51.5699996948242
50 81.4300003051758
100 87.1999969482422
200 89.2900009155273
500 91.3499984741211
1000 92.3099975585938
2000 93.2799987792969
5000 94.5199966430664
5400 94.1699981689453
};
\addplot [very thick, TUMAccentOrange, dotted]
table {%
1 9.81999969482422
2 9.53999996185303
5 9.78999996185303
10 9.97000026702881
20 9.75
50 11.3900003433228
100 21.4300003051758
200 52.6599998474121
500 15.0100002288818
1000 12.8699998855591
2000 93.2600021362305
5000 94.9599990844727
5400 95.2799987792969
};
\addplot [very thick, TUMAccentGreen, loosely dashed]
table {%
1 9.85000038146973
2 9.97000026702881
5 9.8100004196167
10 9.96000003814697
20 10.289999961853
50 13.3900003433228
100 33.6300010681152
200 73.2900009155273
500 92.3099975585938
1000 69.8499984741211
2000 94.129997253418
5000 94.1999969482422
5400 27.1499996185303
};
\nextgroupplot
\addplot [very thick, TUMBlue]
table {%
1 9.92000007629395
2 36.3300018310547
5 51.7200012207031
10 64.0699996948242
20 51.6500015258789
50 81.4199981689453
100 87.1900024414062
200 89.3000030517578
500 91.3499984741211
1000 92.3099975585938
2000 93.2799987792969
5000 94.5199966430664
5400 94.1699981689453
};
\addplot [very thick, TUMAccentOrange, dotted]
table {%
1 9.76000022888184
2 9.34000015258789
5 9.90999984741211
10 10.0299997329712
20 13.25
50 17.6200008392334
100 28.7800006866455
200 71.8300018310547
500 31.2999992370605
1000 22.3299999237061
2000 93.9199981689453
5000 94.9899978637695
5400 95.2799987792969
};
\addplot [very thick, TUMAccentGreen, loosely dashed]
table {%
1 9.82999992370605
2 10.0100002288818
5 9.78999996185303
10 9.90999984741211
20 10.6300001144409
50 27.5799999237061
100 55.6100006103516
200 84.0899963378906
500 92.1999969482422
1000 89.7399978637695
2000 94.1399993896484
5000 95.120002746582
5400 80.6900024414062
};
\nextgroupplot[
ylabel style={rotate=-90},
ytick pos=right,%
ylabel={$\gamma = 10^{-6}$},%
]
\addplot [very thick, TUMBlue]
table {%
1 10.5200004577637
2 46.5800018310547
5 51.6399993896484
10 64.1699981689453
20 51.6500015258789
50 81.4199981689453
100 87.1900024414062
200 89.3000030517578
500 91.3499984741211
1000 92.3099975585938
2000 93.2799987792969
5000 94.5199966430664
5400 94.1699981689453
};
\addplot [very thick, TUMAccentOrange, dotted]
table {%
1 9.85999965667725
2 9.88000011444092
5 9.97999954223633
10 9.80000019073486
20 76.629997253418
50 84.25
100 78.4100036621094
200 89.8600006103516
500 91.6500015258789
1000 92.9400024414062
2000 94.0199966430664
5000 94.9899978637695
5400 95.2799987792969
};
\addplot [very thick, TUMAccentGreen, loosely dashed]
table {%
1 9.97999954223633
2 10
5 10.0200004577637
10 11.460000038147
20 23.6800003051758
50 70.5999984741211
100 87.5100021362305
200 90.9100036621094
500 92.3199996948242
1000 93.0400009155273
2000 94.1399993896484
5000 95.129997253418
5400 95.370002746582
};
\nextgroupplot
\addplot [very thick, TUMBlue]
table {%
1 10.2299995422363
2 9
5 10.1499996185303
10 9.84000015258789
20 16.3199996948242
50 69.6699981689453
100 67.4400024414062
200 88.0100021362305
500 91.5400009155273
1000 92.2300033569336
2000 93.1600036621094
5000 94.2200012207031
5400 94.5
};
\addplot [very thick, TUMAccentOrange, dotted]
table {%
1 9.65999984741211
2 10
5 9.98999977111816
10 9.97999954223633
20 10
50 9.86999988555908
100 10.4399995803833
200 10.2299995422363
500 79.9599990844727
1000 48.0299987792969
2000 25.6000003814697
5000 94.8399963378906
5400 95.379997253418
};
\addplot [very thick, TUMAccentGreen, loosely dashed]
table {%
1 10
2 9.98999977111816
5 10.0100002288818
10 10.1400003433228
20 10.2299995422363
50 10
100 10.1300001144409
200 10.1300001144409
500 14.2700004577637
1000 93.1500015258789
2000 93.9599990844727
5000 94.5400009155273
5400 94.9800033569336
};
\nextgroupplot
\addplot [very thick, TUMBlue]
table {%
1 9.51000022888184
2 10.1999998092651
5 10.9499998092651
10 38.060001373291
20 60.4900016784668
50 81.25
100 87.0899963378906
200 89.6399993896484
500 91.7600021362305
1000 92.2099990844727
2000 93.1900024414062
5000 94.2099990844727
5400 94.5100021362305
};
\addplot [very thick, TUMAccentOrange, dotted]
table {%
1 9.93000030517578
2 9.98999977111816
5 10.1099996566772
10 9.81999969482422
20 10.0600004196167
50 10.1800003051758
100 24.5699996948242
200 28.5699996948242
500 91.7799987792969
1000 49.5400009155273
2000 24.5799999237061
5000 94.8399963378906
5400 95.379997253418
};
\addplot [very thick, TUMAccentGreen, loosely dashed]
table {%
1 9.61999988555908
2 9.97000026702881
5 10
10 10.1800003051758
20 10.3000001907349
50 9.96000003814697
100 10.6899995803833
200 35.2099990844727
500 13.4700002670288
1000 93.120002746582
2000 93.9499969482422
5000 94.5899963378906
5400 94.9599990844727
};
\nextgroupplot
\addplot [very thick, TUMBlue]
table {%
1 10.3999996185303
2 11.8400001525879
5 50.0499992370605
10 38.9700012207031
20 60.8800010681152
50 80.5899963378906
100 87.0699996948242
200 89.6699981689453
500 91.7600021362305
1000 92.2200012207031
2000 93.1800003051758
5000 94.2099990844727
5400 94.5100021362305
};
\addplot [very thick, TUMAccentOrange, dotted]
table {%
1 10.1599998474121
2 10
5 10.0600004196167
10 9.9399995803833
20 10
50 25.2999992370605
100 71.1900024414062
200 63.3199996948242
500 92.1399993896484
1000 50.310001373291
2000 26.6900005340576
5000 94.879997253418
5400 95.379997253418
};
\addplot [very thick, TUMAccentGreen, loosely dashed]
table {%
1 10
2 9.97000026702881
5 10.0100002288818
10 9.72000026702881
20 9.97999954223633
50 9.97000026702881
100 13.9799995422363
200 37.439998626709
500 14.3599996566772
1000 93.120002746582
2000 93.9400024414062
5000 94.6699981689453
5400 95.0699996948242
};
\nextgroupplot
\addplot [very thick, TUMBlue]
table {%
1 11.1599998474121
2 23.9300003051758
5 54.7000007629395
10 39.0499992370605
20 60.8800010681152
50 80.5899963378906
100 87.0800018310547
200 89.6600036621094
500 91.7600021362305
1000 92.2200012207031
2000 93.1800003051758
5000 94.2099990844727
5400 94.5100021362305
};
\addplot [very thick, TUMAccentOrange, dotted]
table {%
1 9.77000045776367
2 10
5 9.89000034332275
10 10.3699998855591
20 10.8299999237061
50 84.5400009155273
100 75.5500030517578
200 78.4100036621094
500 92.1699981689453
1000 67.2699966430664
2000 36.9700012207031
5000 94.9400024414062
5400 95.379997253418
};
\addplot [very thick, TUMAccentGreen, loosely dashed]
table {%
1 9.92000007629395
2 10.0500001907349
5 9.97999954223633
10 9.73999977111816
20 10
50 10.3500003814697
100 15.0799999237061
200 43.9199981689453
500 15.3699998855591
1000 93.120002746582
2000 93.9400024414062
5000 94.8499984741211
5400 95.120002746582
};
\nextgroupplot[
ylabel style={rotate=-90},
ytick pos=right,%
ylabel={$\gamma = 10^{-7}$},%
]
\addplot [very thick, TUMBlue]
table {%
1 10.7600002288818
2 24.1200008392334
5 54.4500007629395
10 39.0400009155273
20 60.8600006103516
50 80.5899963378906
100 87.0800018310547
200 89.6600036621094
500 91.7600021362305
1000 92.2200012207031
2000 93.1800003051758
5000 94.2099990844727
5400 94.5100021362305
};
\addplot [very thick, TUMAccentOrange, dotted]
table {%
1 10.0200004577637
2 10
5 9.94999980926514
10 9.92000007629395
20 48.0200004577637
50 85.870002746582
100 87.8300018310547
200 89.4499969482422
500 92.25
1000 93.2099990844727
2000 93.870002746582
5000 95.129997253418
5400 95.379997253418
};
\addplot [very thick, TUMAccentGreen, loosely dashed]
table {%
1 9.64000034332275
2 10.0299997329712
5 10.0100002288818
10 9.65999984741211
20 10.0200004577637
50 13.0600004196167
100 39.4799995422363
200 88.8899993896484
500 86.6500015258789
1000 93.120002746582
2000 93.9400024414062
5000 94.9700012207031
5400 95.2099990844727
};
\nextgroupplot
\addplot [very thick, TUMBlue]
table {%
1 10.1700000762939
2 10.0600004196167
5 10.1000003814697
10 11.5200004577637
20 13.3900003433228
50 60.0699996948242
100 75.9599990844727
200 87.6100006103516
500 91.0400009155273
1000 92.1699981689453
2000 93.25
5000 94.4800033569336
5400 94.6100006103516
};
\addplot [very thick, TUMAccentOrange, dotted]
table {%
1 10.5699996948242
2 10.2700004577637
5 9.93000030517578
10 10.1099996566772
20 9.98999977111816
50 10.8699998855591
100 10.3000001907349
200 11.1000003814697
500 33.560001373291
1000 45.3199996948242
2000 94.0199966430664
5000 91.4700012207031
5400 95.0699996948242
};
\addplot [very thick, TUMAccentGreen, loosely dashed]
table {%
1 10.3100004196167
2 10.0600004196167
5 10
10 10.039999961853
20 10.1499996185303
50 10.0500001907349
100 9.93000030517578
200 10.7299995422363
500 78.1699981689453
1000 92.9700012207031
2000 14.5799999237061
5000 95.25
5400 26.25
};
\nextgroupplot
\addplot [very thick, TUMBlue]
table {%
1 10.1999998092651
2 9.73999977111816
5 10.3800001144409
10 60.1599998474121
20 60.3199996948242
50 82.5100021362305
100 86.9300003051758
200 89.5899963378906
500 91.3499984741211
1000 92.2699966430664
2000 93.2699966430664
5000 94.4499969482422
5400 94.5800018310547
};
\addplot [very thick, TUMAccentOrange, dotted]
table {%
1 9.76000022888184
2 9.71000003814697
5 9.97000026702881
20 10.0100002288818
50 10.3900003433228
100 11.3800001144409
200 56.9099998474121
500 34.4700012207031
1000 46.4199981689453
2000 94.0500030517578
5000 85.6500015258789
5400 95.0800018310547
};
\addplot [very thick, TUMAccentGreen, loosely dashed]
table {%
1 10.1099996566772
2 10.0699996948242
5 10.0100002288818
10 10.1800003051758
20 10.3900003433228
50 9.92000007629395
100 10.039999961853
200 81.120002746582
500 92.0999984741211
1000 93
2000 14.8299999237061
5000 95.25
5400 27.7999992370605
};
\nextgroupplot
\addplot [very thick, TUMBlue]
table {%
1 10.2799997329712
2 13.0900001525879
5 53.9300003051758
10 60.3199996948242
20 60.4300003051758
50 82.5999984741211
100 86.8899993896484
200 89.5699996948242
500 91.3300018310547
1000 92.2699966430664
2000 93.2699966430664
5000 94.4499969482422
5400 94.5800018310547
};
\addplot [very thick, TUMAccentOrange, dotted]
table {%
1 9.71000003814697
2 9.5600004196167
5 9.96000003814697
10 9.98999977111816
20 10.0799999237061
50 13.0900001525879
100 15.4099998474121
200 55.5
500 34.9000015258789
1000 49.25
2000 94.0299987792969
5000 86.1600036621094
5400 95.0199966430664
};
\addplot [very thick, TUMAccentGreen, loosely dashed]
table {%
1 9.75
2 9.84000015258789
5 10
10 10.1099996566772
20 10
50 10
100 69.2799987792969
200 89.9199981689453
500 92.0800018310547
1000 92.9499969482422
2000 15.1000003814697
5000 95.2600021362305
5400 27.7600002288818
};
\nextgroupplot
\addplot [very thick, TUMBlue]
table {%
1 10.4799995422363
2 37.6100006103516
5 53.7799987792969
10 60.310001373291
20 60.4700012207031
50 82.5899963378906
100 86.9100036621094
200 89.5699996948242
500 91.3300018310547
1000 92.2699966430664
2000 93.2699966430664
5000 94.4499969482422
5400 94.5800018310547
};
\addplot [very thick, TUMAccentOrange, dotted]
table {%
1 9.94999980926514
2 9.85999965667725
5 9.96000003814697
10 9.97000026702881
20 10.0200004577637
50 57.4000015258789
100 15.6400003433228
200 61.7799987792969
500 36.6399993896484
1000 52.75
2000 94.0599975585938
5000 88.4599990844727
5400 95.0599975585938
};
\addplot [very thick, TUMAccentGreen, loosely dashed]
table {%
1 9.85999965667725
2 10.0600004196167
5 10
10 10.1099996566772
20 10.6400003433228
50 12.3900003433228
100 67.7300033569336
200 88.4000015258789
500 92.1500015258789
1000 93.0500030517578
2000 24.2700004577637
5000 95.2600021362305
5400 33.4700012207031
};
\nextgroupplot[
ylabel style={rotate=-90},
ytick pos=right,%
ylabel={$\gamma = 10^{-8}$},%
]
\addplot [very thick, TUMBlue]
table {%
1 13.6999998092651
2 43.4000015258789
5 53.8899993896484
10 60.3400001525879
20 60.4700012207031
50 82.5899963378906
100 86.9100036621094
200 89.5699996948242
500 91.3300018310547
1000 92.2699966430664
2000 93.2699966430664
5000 94.4499969482422
5400 94.5800018310547
};
\addplot [very thick, TUMAccentOrange, dotted]
table {%
1 9.43000030517578
2 10.289999961853
5 9.93000030517578
10 9.96000003814697
20 10.3100004196167
50 69.1900024414062
100 22.9500007629395
200 86.9700012207031
500 63.4900016784668
1000 91.1699981689453
2000 94.129997253418
5000 94.5999984741211
5400 95.1399993896484
};
\addplot [very thick, TUMAccentGreen, loosely dashed]
table {%
1 10.1099996566772
2 9.96000003814697
5 10
10 10.0500001907349
20 28.1200008392334
50 15.0500001907349
100 77.5899963378906
200 89.6800003051758
500 92.629997253418
1000 93.0899963378906
2000 79.9199981689453
5000 95.2600021362305
5400 80.7900009155273
};
\nextgroupplot
\addplot [very thick, TUMBlue]
table {%
1 10.2399997711182
2 9.81999969482422
5 10.2700004577637
10 10.4200000762939
20 11.5500001907349
50 28.1599998474121
100 70.6100006103516
200 85.879997253418
500 91.5
1000 92.1900024414062
2000 93.4499969482422
5000 94.5999984741211
5400 94.620002746582
};
\addplot [very thick, TUMAccentOrange, dotted]
table {%
1 10.0699996948242
2 10.9300003051758
5 10.2700004577637
10 9.77999973297119
20 10
50 9.63000011444092
100 9.90999984741211
200 10.3000001907349
500 39.4300003051758
1000 92.2600021362305
2000 71.9100036621094
5000 94.75
5400 95.2399978637695
};
\addplot [very thick, TUMAccentGreen, loosely dashed]
table {%
1 9.9399995803833
2 10.0299997329712
5 10
10 10
20 10.0200004577637
50 9.61999988555908
100 10.1899995803833
200 10.1899995803833
500 20.8899993896484
1000 92.1600036621094
2000 94.1699981689453
5000 95.0199966430664
5400 95.0100021362305
};
\nextgroupplot
\addplot [very thick, TUMBlue]
table {%
1 10.4700002670288
2 10.0200004577637
5 10.460000038147
10 56.5299987792969
20 63.4099998474121
50 83.0699996948242
100 86.8399963378906
200 89.4100036621094
500 91.4800033569336
1000 92.1999969482422
2000 93.4400024414062
5000 94.5899963378906
5400 94.629997253418
};
\addplot [very thick, TUMAccentOrange, dotted]
table {%
1 10.1400003433228
2 10
5 10.1499996185303
10 9.67000007629395
20 10
50 10.5699996948242
100 31.4500007629395
200 10.7200002670288
500 11.2399997711182
1000 92.5100021362305
2000 52.1100006103516
5000 94.8399963378906
5400 95.2099990844727
};
\addplot [very thick, TUMAccentGreen, loosely dashed]
table {%
1 10.460000038147
2 10.1999998092651
5 9.98999977111816
20 10.0100002288818
50 10.3000001907349
100 26.3799991607666
200 13.6800003051758
500 23.8099994659424
1000 92.379997253418
2000 94.2099990844727
5000 94.9499969482422
5400 94.9300003051758
};
\nextgroupplot
\addplot [very thick, TUMBlue]
table {%
1 10.3500003814697
2 19.9400005340576
5 34.1800003051758
10 56.9700012207031
20 62.4199981689453
50 83.120002746582
100 86.8600006103516
200 89.4400024414062
500 91.4800033569336
1000 92.1999969482422
2000 93.4400024414062
5000 94.5899963378906
5400 94.629997253418
};
\addplot [very thick, TUMAccentOrange, dotted]
table {%
1 9.89999961853027
2 9.98999977111816
5 9.84000015258789
10 10.1700000762939
20 10.0600004196167
50 10.4499998092651
100 87.4100036621094
200 13.960000038147
500 10.0100002288818
1000 92.5999984741211
2000 21.4200000762939
5000 94.7399978637695
5400 95.2099990844727
};
\addplot [very thick, TUMAccentGreen, loosely dashed]
table {%
1 10.1099996566772
2 9.88000011444092
5 10
10 9.98999977111816
20 10.1099996566772
50 12.75
100 57.3199996948242
200 24.9699993133545
500 25.1200008392334
1000 92.2099990844727
2000 94.2200012207031
5000 94.9300003051758
5400 94.8899993896484
};
\nextgroupplot
\addplot [very thick, TUMBlue]
table {%
1 10.4499998092651
2 37.3600006103516
5 47.9500007629395
10 56.9700012207031
20 62.3199996948242
50 83.120002746582
100 86.8600006103516
200 89.4400024414062
500 91.4899978637695
1000 92.1999969482422
2000 93.4400024414062
5000 94.5899963378906
5400 94.629997253418
};
\addplot [very thick, TUMAccentOrange, dotted]
table {%
1 9.60999965667725
2 10
5 9.56999969482422
10 9.97999954223633
20 10.0100002288818
50 17.25
100 87.4499969482422
200 11.289999961853
500 10.0299997329712
1000 92.4499969482422
2000 21.4699993133545
5000 94.7799987792969
5400 95.2099990844727
};
\addplot [very thick, TUMAccentGreen, loosely dashed]
table {%
1 10.1199998855591
2 10.3400001525879
5 10
10 9.97999954223633
20 9.88000011444092
50 79.8199996948242
100 59.189998626709
200 23.2900009155273
500 23.8199996948242
1000 92.6600036621094
2000 94.2200012207031
5000 95
5400 94.9599990844727
};
\nextgroupplot[
ylabel style={rotate=-90},
ytick pos=right,%
ylabel={$\gamma = 10^{-9}$},%
]
\addplot [very thick, TUMBlue]
table {%
1 9.02999973297119
2 38.1199989318848
5 48.0699996948242
10 56.9700012207031
20 62.4199981689453
50 83.120002746582
100 86.8600006103516
200 89.4400024414062
500 91.4899978637695
1000 92.1999969482422
2000 93.4400024414062
5000 94.5899963378906
5400 94.629997253418
};
\addplot [very thick, TUMAccentOrange, dotted]
table {%
1 9.84000015258789
2 10
5 10
10 10.1000003814697
20 14.6800003051758
50 23.4699993133545
100 88.3899993896484
200 11.1099996566772
500 10.0500001907349
1000 92.6500015258789
2000 39.7299995422363
5000 94.7799987792969
5400 95.2099990844727
};
\addplot [very thick, TUMAccentGreen, loosely dashed]
table {%
1 10.0699996948242
2 10.1899995803833
5 10
10 9.80000019073486
20 16.5699996948242
50 81.9499969482422
100 69.6500015258789
200 23.5699996948242
500 35.1699981689453
1000 92.9199981689453
2000 94.2200012207031
5000 95.0500030517578
5400 95
};
\end{groupplot}
\path (group c1r8.south east) -- node[below=1.2cm]{\pgfplotslegendfromname{LegendSmallData}} (group c5r8.south west);
\end{tikzpicture}

\end{document}
