# Supplementary material for: Learning Expressive Priors for Generalization and Uncertainty Estimation in Neural Networks
Source: arXiv:2307.07753 source file (2026-03-30)
Supplement: Supplementary file 6 [file skp_isotropic.tex]

\documentclass{standalone}
\usepackage[ansinew]{inputenc}

\usepackage{../../tikz_include}

\begin{document}

\begin{tikzpicture}

% power method 0.01020 \pm 0.03129
% sum 0.10167 \pm 0.22935

\begin{groupplot}[
    footnotesize,
    %width=0.5\columnwidth,
    %height=0.3\columnwidth,
    group style={group size=4 by 1, y descriptions at=edge left, x descriptions at=edge bottom},
    log basis y={10},
    ylabel={Relative error},
    ymode=log,
    max space between ticks=30pt,
    ]
    \nextgroupplot[
    legend to name={LegendAblations},
    legend style={legend columns=2}, 
    xlabel={Size of the matrices $M=N$}
    ]
        \path [draw=TUMAccentOrange, fill=TUMAccentOrange, opacity=0.2]
(axis cs:2,0.122519445456618)
--(axis cs:2,0.11217354340406)
--(axis cs:3,0.102707662526528)
--(axis cs:4,0.0979445677221596)
--(axis cs:5,0.0972459958845971)
--(axis cs:6,0.0967570388466431)
--(axis cs:7,0.0974619036010183)
--(axis cs:8,0.0973784399288036)
--(axis cs:9,0.0974543706486668)
--(axis cs:10,0.0972605563888383)
--(axis cs:11,0.0967748747399673)
--(axis cs:12,0.096346468997471)
--(axis cs:13,0.0962050045378822)
--(axis cs:14,0.0955431475890601)
--(axis cs:15,0.0953737444835598)
--(axis cs:16,0.0948585369226398)
--(axis cs:17,0.094812314351928)
--(axis cs:18,0.0940735141920699)
--(axis cs:19,0.0939019243934296)
--(axis cs:19,0.10232970281399)
--(axis cs:19,0.10232970281399)
--(axis cs:18,0.102583842945261)
--(axis cs:17,0.102685756819855)
--(axis cs:16,0.103151269420594)
--(axis cs:15,0.103497014649711)
--(axis cs:14,0.104091981312271)
--(axis cs:13,0.104281441602981)
--(axis cs:12,0.104623786705543)
--(axis cs:11,0.104783301058989)
--(axis cs:10,0.106021029059163)
--(axis cs:9,0.105616655675487)
--(axis cs:8,0.106265894355935)
--(axis cs:7,0.105410598834249)
--(axis cs:6,0.104993230786945)
--(axis cs:5,0.105688693281875)
--(axis cs:4,0.107092067446272)
--(axis cs:3,0.11168197800059)
--(axis cs:2,0.122519445456618)
--cycle;

\path [draw=TUMBlue, fill=TUMBlue, opacity=0.2]
(axis cs:2,0.00727942811941512)
--(axis cs:2,0.00642017944251745)
--(axis cs:3,0.00843523795717179)
--(axis cs:4,0.00904032316581011)
--(axis cs:5,0.00950774343177528)
--(axis cs:6,0.00986333808834376)
--(axis cs:7,0.0101713546906818)
--(axis cs:8,0.0104108406526779)
--(axis cs:9,0.0103497563831788)
--(axis cs:10,0.0102398088233816)
--(axis cs:11,0.0100186628330287)
--(axis cs:12,0.009950900166723)
--(axis cs:13,0.00995275853377395)
--(axis cs:14,0.0099247529701048)
--(axis cs:15,0.00984924474926948)
--(axis cs:16,0.00984640436627141)
--(axis cs:17,0.00982096400985531)
--(axis cs:18,0.00983534986413616)
--(axis cs:19,0.00983990933391216)
--(axis cs:19,0.0110745143261731)
--(axis cs:19,0.0110745143261731)
--(axis cs:18,0.0110707036021174)
--(axis cs:17,0.0110630455364607)
--(axis cs:16,0.0109980451321899)
--(axis cs:15,0.0109723099745768)
--(axis cs:14,0.0110753096649742)
--(axis cs:13,0.010997069245972)
--(axis cs:12,0.0111232378316728)
--(axis cs:11,0.0112369569007491)
--(axis cs:10,0.0114316356131214)
--(axis cs:9,0.0115411951166504)
--(axis cs:8,0.0116160598279252)
--(axis cs:7,0.0114046966894963)
--(axis cs:6,0.0110461652199009)
--(axis cs:5,0.0105943295377921)
--(axis cs:4,0.0100788140084504)
--(axis cs:3,0.00943863552071243)
--(axis cs:2,0.00727942811941512)
--cycle;

\addplot [very thick, TUMAccentOrange, dotted]
table {%
2 0.117359779775143
3 0.107098817825317
4 0.102358065545559
5 0.101466372609138
6 0.100831739604473
8 0.101897649466991
9 0.101597025990486
10 0.101472586393356
11 0.100654318928719
13 0.100175522267818
14 0.0998386740684509
15 0.0992229357361794
16 0.0990400537848473
18 0.0984412059187889
19 0.0979265347123146
};
%\addlegendentry{Sum}
\addplot [very thick, TUMBlue]
table {%
2 0.00685918796807528
3 0.00891984719783068
4 0.00953147374093533
5 0.0100155184045434
6 0.0104451477527618
7 0.0107878446578979
8 0.0109677398577332
9 0.0109123745933175
10 0.0108228689059615
11 0.0106102610006928
12 0.0105324434116483
13 0.010500269010663
14 0.0104835936799645
15 0.01041797734797
16 0.0104163018986583
17 0.0104519994929433
19 0.0104445368051529
};
\addlegendentry{Sum}

\addlegendentry{Power method}
%\addlegendentry{Power method}

    \nextgroupplot[
    xlabel={Scale of the Fisher matrix},
    log basis x={10},
    xmode=log
    ]
\path [draw=TUMAccentOrange, fill=TUMAccentOrange, opacity=0.2]
(axis cs:9.99999974737875e-06,0.15949104815747)
--(axis cs:9.99999974737875e-06,0.153117476699692)
--(axis cs:9.99999974737875e-05,0.221730644184837)
--(axis cs:0.00100000004749745,0.231097612618991)
--(axis cs:0.00999999977648258,0.221618860527023)
--(axis cs:0.100000001490116,0.138028521710087)
--(axis cs:1,0.0266214179559934)
--(axis cs:10,0.0027676806279262)
--(axis cs:100,0.000286831375106288)
--(axis cs:1000,3.02719686370979e-05)
--(axis cs:10000,2.8883829246082e-06)
--(axis cs:10000,3.33027983448225e-06)
--(axis cs:10000,3.33027983448225e-06)
--(axis cs:1000,3.8910745818821e-05)
--(axis cs:100,0.000335476267170331)
--(axis cs:10,0.0031008283840438)
--(axis cs:1,0.0296052220449408)
--(axis cs:0.100000001490116,0.145586506676433)
--(axis cs:0.00999999977648258,0.230251148489612)
--(axis cs:0.00100000004749745,0.239782700668611)
--(axis cs:9.99999974737875e-05,0.230071238274465)
--(axis cs:9.99999974737875e-06,0.15949104815747)
--cycle;

\path [draw=TUMBlue, fill=TUMBlue, opacity=0.2]
(axis cs:9.99999974737875e-06,0.0165306621593339)
--(axis cs:9.99999974737875e-06,0.0156219075265511)
--(axis cs:9.99999974737875e-05,0.0224325211585872)
--(axis cs:0.00100000004749745,0.0231808373290533)
--(axis cs:0.00999999977648258,0.0230477103542872)
--(axis cs:0.100000001490116,0.0139305872694702)
--(axis cs:1,0.000879822772653518)
--(axis cs:10,1.17879351739696e-05)
--(axis cs:100,2.19110369342283e-07)
--(axis cs:1000,9.97547452940425e-08)
--(axis cs:10000,9.86456361486534e-08)
--(axis cs:10000,1.00031716983231e-07)
--(axis cs:10000,1.00031716983231e-07)
--(axis cs:1000,1.01356290865702e-07)
--(axis cs:100,2.85406080057958e-07)
--(axis cs:10,1.76825641832699e-05)
--(axis cs:1,0.00106245308189574)
--(axis cs:0.100000001490116,0.0149630587176351)
--(axis cs:0.00999999977648258,0.0242769070532058)
--(axis cs:0.00100000004749745,0.0244609756343751)
--(axis cs:9.99999974737875e-05,0.0236379138783032)
--(axis cs:9.99999974737875e-06,0.0165306621593339)
--cycle;

\addplot [very thick, TUMAccentOrange, dotted]
table {%
9.99998883344233e-06 0.156207799911499
9.99999974737875e-05 0.225641176104546
0.000999999465420842 0.235772371292114
0.00999999418854713 0.225922420620918
0.100000001490116 0.141840279102325
1 0.0280060842633247
10 0.00292558851651847
100.000053405762 0.000309999100863934
1000.00054931641 3.39839862135705e-05
10000 3.10000973513525e-06
};
\addplot [very thick, TUMBlue]
table {%
9.99998883344233e-06 0.0160848349332809
9.99999974737875e-05 0.0230251085013151
0.000999999465420842 0.0238454043865204
0.00999999418854713 0.0236268881708384
0.100000001490116 0.0144133623689413
1 0.000969854823779315
10 1.44384675877518e-05
100.000053405762 2.49558013365458e-07
1000.00054931641 1.00592338014849e-07
10000 9.93396795934132e-08
};

    \nextgroupplot[
    xlabel={Weight decay $\gamma$},
    log basis x={10},
    xmode=log
    ]
\path [draw=TUMAccentOrange, fill=TUMAccentOrange, opacity=0.2]
(axis cs:1.00000001335143e-10,0.00800384564081939)
--(axis cs:1.00000001335143e-10,0.00748036735254617)
--(axis cs:9.99999971718069e-10,0.0233749677630515)
--(axis cs:9.99999993922529e-09,0.0661440773135691)
--(axis cs:1.0000000116861e-07,0.107579103557585)
--(axis cs:9.99999997475243e-07,0.122682268287629)
--(axis cs:9.99999974737875e-06,0.126492794872407)
--(axis cs:9.99999974737875e-05,0.126154131839957)
--(axis cs:0.00100000004749745,0.126219770078045)
--(axis cs:0.00999999977648258,0.125812794531712)
--(axis cs:0.100000001490116,0.126845518078519)
--(axis cs:1,0.126743559755679)
--(axis cs:1,0.133830067244778)
--(axis cs:1,0.133830067244778)
--(axis cs:0.100000001490116,0.134500472906008)
--(axis cs:0.00999999977648258,0.13337201661712)
--(axis cs:0.00100000004749745,0.133913409809404)
--(axis cs:9.99999974737875e-05,0.133413637672231)
--(axis cs:9.99999974737875e-06,0.133861408031326)
--(axis cs:9.99999997475243e-07,0.129946500371253)
--(axis cs:1.0000000116861e-07,0.114584095151212)
--(axis cs:9.99999993922529e-09,0.0708711824254153)
--(axis cs:9.99999971718069e-10,0.025064986943017)
--(axis cs:1.00000001335143e-10,0.00800384564081939)
--cycle;

\path [draw=TUMBlue, fill=TUMBlue, opacity=0.2]
(axis cs:1.00000001335143e-10,0.000138007772286905)
--(axis cs:1.00000001335143e-10,0.000126575694019881)
--(axis cs:9.99999971718069e-10,0.00115574957699472)
--(axis cs:9.99999993922529e-09,0.0070916500617298)
--(axis cs:1.0000000116861e-07,0.0114156686148012)
--(axis cs:9.99999997475243e-07,0.0124881879860005)
--(axis cs:9.99999974737875e-06,0.0126900314337843)
--(axis cs:9.99999974737875e-05,0.0125848797075437)
--(axis cs:0.00100000004749745,0.0125456998778994)
--(axis cs:0.00999999977648258,0.0125705089965836)
--(axis cs:0.100000001490116,0.012550365063812)
--(axis cs:1,0.012580335158)
--(axis cs:1,0.0135925367383384)
--(axis cs:1,0.0135925367383384)
--(axis cs:0.100000001490116,0.0135858048266453)
--(axis cs:0.00999999977648258,0.0136421512112014)
--(axis cs:0.00100000004749745,0.0135529175736348)
--(axis cs:9.99999974737875e-05,0.0136578802637709)
--(axis cs:9.99999974737875e-06,0.0137090225558173)
--(axis cs:9.99999997475243e-07,0.0135257228799567)
--(axis cs:1.0000000116861e-07,0.0122832811125334)
--(axis cs:9.99999993922529e-09,0.0077446496317379)
--(axis cs:9.99999971718069e-10,0.00126018585477271)
--(axis cs:1.00000001335143e-10,0.000138007772286905)
--cycle;

\addplot [very thick, TUMAccentOrange, dotted]
table {%
9.99997792905383e-11 0.00773275131359696
9.99999971718069e-10 0.0241776145994663
9.9999777347648e-09 0.0684606060385704
9.9999887481772e-08 0.111149370670319
9.99998860606865e-07 0.126350447535515
9.99998883344233e-06 0.130162164568901
9.99999974737875e-05 0.129636883735657
0.000999999465420842 0.130178287625313
0.00999999418854713 0.129693582653999
0.100000001490116 0.130434811115265
1 0.130352601408958
};
\addplot [very thick, TUMBlue]
table {%
9.99997792905383e-11 0.000131806242279708
9.99999971718069e-10 0.00120960350614041
9.9999777347648e-09 0.00740867806598544
9.9999887481772e-08 0.0118495272472501
9.99998860606865e-07 0.0130121950060129
9.99998883344233e-06 0.0131593504920602
0.000999999465420842 0.0130519764497876
0.100000001490116 0.0130749037489295
1 0.0130970738828182
};

    \nextgroupplot[
    %xlabel={Weight decay $\gamma$},
    %log basis x={10},
    %xmode=log
    %legend pos=middle east,
    log basis y={10},
    xlabel={Number of matrices $K$},
    ymode=log,
    ]

\path [draw=TUMAccentOrange, fill=TUMAccentOrange, opacity=0.2]
(axis cs:2,1.03864355260134)
--(axis cs:2,0.9853386426121)
--(axis cs:3,1.87895284417272)
--(axis cs:4,2.78600546628237)
--(axis cs:5,3.75371983194351)
--(axis cs:6,4.63441372185946)
--(axis cs:7,5.62662349140644)
--(axis cs:8,6.56534879124165)
--(axis cs:9,7.60414712679386)
--(axis cs:9,7.69065375852585)
--(axis cs:9,7.69065375852585)
--(axis cs:8,6.65625695133209)
--(axis cs:7,5.72423603761196)
--(axis cs:6,4.72003535586596)
--(axis cs:5,3.83988089162111)
--(axis cs:4,2.87205077725649)
--(axis cs:3,1.94894404053688)
--(axis cs:2,1.03864355260134)
--cycle;

\path [draw=TUMBlue, fill=TUMBlue, opacity=0.2]
(axis cs:2,0.283380622072145)
--(axis cs:2,0.252634905166924)
--(axis cs:3,0.297439105752856)
--(axis cs:4,0.307871565226465)
--(axis cs:5,0.307534970406443)
--(axis cs:6,0.296102681148797)
--(axis cs:7,0.290397300831974)
--(axis cs:8,0.280523322787136)
--(axis cs:9,0.272456125639379)
--(axis cs:9,0.284319386590272)
--(axis cs:9,0.284319386590272)
--(axis cs:8,0.292414742611349)
--(axis cs:7,0.304976718049496)
--(axis cs:6,0.311138603907078)
--(axis cs:5,0.325094482898712)
--(axis cs:4,0.32630025895685)
--(axis cs:3,0.320748204290867)
--(axis cs:2,0.283380622072145)
--cycle;

\addplot [very thick, TUMAccentOrange, dotted]
table {%
2 1.01334500312805
3 1.91478598117828
4 2.82916951179504
5 3.79627466201782
6 4.67773628234863
7 5.67293787002563
8 6.61105346679688
9 7.64502191543579
};
\addplot [very thick, TUMBlue]
table {%
2 0.267955362796783
3 0.309673100709915
4 0.316953808069229
5 0.316233664751053
6 0.30384173989296
7 0.297444760799408
8 0.28637620806694
9 0.277988106012344
};

\end{groupplot}

    \path (group c1r1.east) -- node[left=-1cm]{\pgfplotslegendfromname{LegendAblations}} (group c1r1.east);
\end{tikzpicture}
\noindent
\end{document}
