# Supplementary material for: Learning Expressive Priors for Generalization and Uncertainty Estimation in Neural Networks
Source: arXiv:2307.07753 source file (2026-03-30)
Supplement: Supplementary file 7 [file skp_multiple_matrices.tex]

\documentclass{standalone}
\usepackage[ansinew]{inputenc}

\usepackage{../../tikz_include}

\begin{document}

\begin{tikzpicture}

\begin{axis}[
legend pos=north west,
log basis y={10},
xlabel={Number of matrices $K$},
ylabel={Relative Error},
ymode=log,
]
\path [draw=TUMAccentOrange, fill=TUMAccentOrange, opacity=0.2]
(axis cs:2,1.03864355260134)
--(axis cs:2,0.9853386426121)
--(axis cs:3,1.87895284417272)
--(axis cs:4,2.78600546628237)
--(axis cs:5,3.75371983194351)
--(axis cs:6,4.63441372185946)
--(axis cs:7,5.62662349140644)
--(axis cs:8,6.56534879124165)
--(axis cs:9,7.60414712679386)
--(axis cs:9,7.69065375852585)
--(axis cs:9,7.69065375852585)
--(axis cs:8,6.65625695133209)
--(axis cs:7,5.72423603761196)
--(axis cs:6,4.72003535586596)
--(axis cs:5,3.83988089162111)
--(axis cs:4,2.87205077725649)
--(axis cs:3,1.94894404053688)
--(axis cs:2,1.03864355260134)
--cycle;

\path [draw=TUMBlue, fill=TUMBlue, opacity=0.2]
(axis cs:2,0.283380622072145)
--(axis cs:2,0.252634905166924)
--(axis cs:3,0.297439105752856)
--(axis cs:4,0.307871565226465)
--(axis cs:5,0.307534970406443)
--(axis cs:6,0.296102681148797)
--(axis cs:7,0.290397300831974)
--(axis cs:8,0.280523322787136)
--(axis cs:9,0.272456125639379)
--(axis cs:9,0.284319386590272)
--(axis cs:9,0.284319386590272)
--(axis cs:8,0.292414742611349)
--(axis cs:7,0.304976718049496)
--(axis cs:6,0.311138603907078)
--(axis cs:5,0.325094482898712)
--(axis cs:4,0.32630025895685)
--(axis cs:3,0.320748204290867)
--(axis cs:2,0.283380622072145)
--cycle;

\addplot [very thick, TUMAccentOrange]
table {%
2 1.01334500312805
3 1.91478598117828
4 2.82916951179504
5 3.79627466201782
6 4.67773628234863
7 5.67293787002563
8 6.61105346679688
9 7.64502191543579
};
\addlegendentry{Sum}
\addplot [very thick, TUMBlue]
table {%
2 0.267955362796783
3 0.309673100709915
4 0.316953808069229
5 0.316233664751053
6 0.30384173989296
7 0.297444760799408
8 0.28637620806694
9 0.277988106012344
};
\addlegendentry{Power method}
\end{axis}

\end{tikzpicture}

\end{document}
